# Supplementary material for: BrainLLM: Generative Language Decoding from Brain Recordings
Source: arXiv:2311.09889 source file (2025-11-02)
Supplement: Supplementary file 1 [file SI.pdf]

# Supplementary Information to "Generative Language Reconstruction from Brain Recordings"

## A Materials

Three publicly available functional magnetic resonance imaging (fMRI) datasets are used in the experiments:: Pereira's dataset [1], Huth's dataset [2], and the Narratives dataset [3]. The statistics of these datasets are listed in Table 20. The scope of our current study focuses on non-invasive fMRI data collected during participants perceiving (listening or reading) natural language sequence. Other types of brain signals, such as brain signals collected from invasive devices with higher resolution, and non-invasive signals such as MEG and EEG, were not investigated in this study. Nonetheless, we believe that generative-based language decoding methods could be applied to these signals in future research.

### A.1 Pereira's dataset

Pereira's dataset [1] consists of recordings from 16 participants' fMRI data while they are watching visual content comprising single words and sentences structured in a style akin to Wikipedia. There are data from three fMRI experiments in their study. We selected data from experiments 2 and 3, in which participants were asked to watch the sentence-based visual contents attentively, with each sentence in the passage presented at one time. To mitigate the overlap issue of BOLD signals between adjacent stimuli, a four-second fixation period was implemented following the presentation of each sentence. Structural and functional MRI data were collected on a whole-body 3-Tesla Siemens Trio scanner with a 32-channel head coil at the Athinoula A. Martinos Imaging Center at the McGovern Institute for Brain Research at MIT or at the Scully Center for the Neuroscience of Mind and Behavior at Princeton University. Each participant did 3 repetitions for each sentence and the averaged beta coefficient brain images (see the original paper [1] for the definition of beta coefficient brain images) corresponding to each sentence are adopted as brain input in our study. Consistent with previous work focusing on sentence decoding [4], the cognitive data of participants who both participated in experiments 2 and 3 were selected in this paper. In summary, experiments 2 and 3 involved five participants who each responded to 168 passages, with an average of 3.7 sentences per passage.

We use the officially pre-processed beta coefficient images released in the dataset's website (https://osf.io/crwz7). Structural and functional MRI data were analyzed using FSL (http://fsl.fmrib.ox.ac.uk/fsl/) and custom MATLAB scripts. The fMRI data from each scanning session underwent slice timing correction, motion correction, bias field inhomogeneity correction, and high-pass filtering (cutoff: 100 seconds).

### A.2 Huth's dataset

Huth's dataset [2], also known as the natural language dataset, contains BOLD fMRI responses recorded from 8 participants each listening to 27 complete, natural, narrative stories (6 hours in total). The stories were sourced from podcasts, including "The Moth Radio Hour," "Modern Love," and "The Anthropocene Reviewed." Each story, lasting approximately 10-15 minutes, was presented during a separate fMRI scan. Participants were instructed to listen to the stories attentively and were not required to provide any responses.

At the same time, the MRI data were collected on a 3T Siemens Skyra scanner at The University of Texas at Austin Biomedical Imaging Center using a 64-channel Siemens volume coil.

We use the officially pre-processed version of the dataset. Each functional run underwent motion correction using the FMRIB Linear Image Registration Tool (FLIRT) followed by averaging to generate a high-quality template volume. In the user experiment of Huth's dataset, BOLD signals are collected synchronously with the auditory stimulus presentation. Hence, it is imperative to account for the delay effect inherent in the BOLD signals. In alignment with established precedents in previous research, we consider the 1st to 4th post-stimulus TR periods as the window for capturing the participant's neural response to the stimulus. To mitigate the effects of onset artifacts and suboptimal detrending at the scan's beginning and end, the first and last 5 TRs of each story are removed. As a result, each participant had 9,244 TRs of functional data.

## A.3 Narratives dataset

The "Narratives" dataset collection aggregates a variety of fMRI datasets collected while human participants listened to naturalistic spoken stories. The dataset includes 345 participants, 891 functional scans, and 27 diverse stories of varying duration totaling 4.6 hours of unique stimuli. Story stimuli encompass a diverse range of media, including commercially produced radio and internet broadcasts, readings of written works, live performances by professional storytellers, etc. Similar to the collection procedures used in Huth's dataset, participants were instructed to listen to the stories attentively and were not required to provide any responses. All MRI data were collected at the Princeton Neuroscience Institute Scully Center for Neuroimaging. The MRI devices include two 3 T Siemens Magnetom Prisma each with a 64-channel head coil. The vast majority of participants only participated in one fMRI experiment, so the average scan duration for each participant was only 21 minutes. However, some participants engaged in multiple scans, contributing to a larger number of MRI data samples for the training the language generation experiments in a within-participant setup. Therefore, we selected all participants in the Narratives dataset who had participated in at least three fMRI scans for our experiment. This criterion selects 28 participants whose ids are: sub-016,sub-026,sub-034,sub-041,sub-052,sub-055,sub-058,sub-059,sub-060,sub-061,sub-065,sub-066,sub-075,sub-084,sub-106,sub-111,sub-132,sub-133,sub-134,sub-135,sub-136,sub-137,sub-140,sub-141,sub-142,sub-143,sub-144, and sub-145.

The "Narrative" fMRI dataset was released with various preprocessed versions, e.g., AFNI-smooth, AFNI. We use the AFNI-smooth version of the released data. Similar to the pre-processing of Huth's dataset, we treat the 1-st to 4-th TR after a user receives a stimulus as the response. For the fMRI sequence of a participant, the volumes before the onset and after the end of the story stimuli are discarded. The time series of each voxel is normalized to have zero mean and unit standard deviation.

## A.4 Comparative analysis of different datasets

Huth's dataset and the Narratives dataset use similar settings such as the selection of natural story stimuli, experimental task description, etc. However, the statistics of the natural language dataset and the Narratives dataset are quite different. The Narratives dataset contains neuroimaging data from a large number of participants, i.e., 345, but the data collected from each participant is only 21 minutes on average. On the other hand, Huth's dataset involves only 8 participants, but the recorded time is much longer than that in the Narratives dataset, i.e., 6 hours for each participant. Therefore, we conducted experiments to analyze the effect of different training data sizes on the model performance within Huth's dataset and the Narratives dataset. We found that the average performance in terms of win rate of BrainLLM versus PerBrainLLM of the two datasets was very close when using the same training data size (see Main Paper Fig. 2(f)). However, as Huth's dataset contains more data samples, the averaged performance in Huth's dataset is better than that in the Narratives dataset when using all data for training.

On the other hand, Pereira's dataset exhibits several distinct characteristics when compared with Huth's dataset and the Narratives dataset. The major differences include the employment of visual stimuli, the non-continuous presentation of stimulation, and the utilization of diverse language styles. Based on these differences, we also extract different features from fMRI signals as input for BrainLLM, i.e., beta coefficients

for Pereira's dataset and raw BOLD signals for Huth's and Narratives datasets. This issue arises due to the Huth and Narratives datasets, where stimuli are presented continuously without clear temporal boundaries. Such continuous presentation may violate the assumption of residual independence required by GLMs, resulting in inaccurate modeling when using the hemodynamic response function (HRF) for convolution.

We observe that the performance metrics associated with Pereira's dataset diverge significantly from those observed in Huth's and the Narratives dataset, even with the same training data size (see Main Paper Fig. 2(f)). This variation in performance can primarily be attributed to the disparate settings employed in Pereira's datasets.

# B Methods

## B.1 Illustration and discussion for experimental dataset construction

We constructed the data samples for the language generation task with the blood oxygen level dependent (BOLD) features, corresponding stimuli presented to the participant (perceived continuation), and the text prompt (if any) that preceded the stimuli. For Pereira's dataset, brain responses are collected within the corresponding time frames for each sentence. Notably, each sentence is presented three times, and the averaged signals are utilized for analysis (for detailed experimental settings, refer to the original paper [1]). We split the sentence $P$ corresponding to the fMRI signals into three parts with equal length, i.e., $P_1$, $P_2$, and $P_3$. Two unique data samples are generated by treating the first third ($P_1$) as the text prompt and the second third ($P_2$) as the perceived continuation as well as combining the first two-thirds ($P_1$ and $P_2$) as the text prompt and using the last third ($P_3$) as the perceived continuation. At the same time, the brain response to sentence $P$ is adopted for generating the perceived continuation with BrainLLM in these two data samples. The construction of such data samples serves three primary objectives. First, it allows the model to adapt to text prompts of different lengths, so that we can study the impact of prompt length and surprise levels on the language generation performance with BrainLLM. Second, it allows us to construct as many data samples as possible with limited data. Last, segmenting the data into three parts allows the perceived continuation to be distributed between 3 and 10 words, which is consistent with the settings of Huth's dataset and the Narratives dataset that will be introduced later.

For Huth's and the Narratives dataset, the language stimuli were presented to the participants continuously. Therefore, we split the dataset according to the TRs (2s in Huth's dataset and 1.5s in the Narratives dataset). The BOLD features and the corresponding perceived continuation are first selected from each TR. Then we used a slide window ranging from 1 to 3 TRs to pick the language stimuli before the perceived continuation appeared as the text prompt. This step constructed 3 data samples for each TR. This is an example of how we construct the data samples for Huth's dataset and the Narratives dataset. Given a series of TRs, i.e., $TR_1$, $TR_2$, $TR_3$, $TR_4$, $\ldots$, $TR_n$, and the corresponding language stimuli $P_i$ for each $TR_i$ ($i \in \{1, 2, \ldots, n\}$), we generate a series of decoding tasks including:

- $\{W = P_1, M = P_2\}$; $\{W = P_2, M = P_3\}$;$\{W = P_3, M = P_4]\}$; ...
- $\{W = \text{concatenate}(P_1, P_2), M = P_3\}$; $\{W = \text{concatenate}(P_2, P_3), M = P_4]\}$; ...
- $\{W = \text{concatenate}(P_1, P_2, P_3), M = P_4\}$; $\{W = \text{concatenate}(P_2, P_3, P_4), M = P_5\}$; ...

where $W$ is the text prompt and $M$ is the perceived continuation that we aim to generate. Similarly, the construction of data samples aims to create as many samples as possible with limited neurological data and ensure that the model is adept at handling text prompts of varying lengths.

After that, the constructed data samples are split using a split-by-stimuli protocol. The stimuli (i.e., perceived continuation) as well as its corresponding brain recordings are randomly shuffled and split into training, validation, and test sets with a size roughly proportional to 3:1:1, respectively. The splitting ensured that there was no overlap of perceived continuation and brain recordings among the training, validation, and test sets. Besides this split-by-stimuli protocol, we also test the split-by-story splitting protocol in Huth's dataset (Huth's data set contains 27 stories as stimuli for each participant and thus is more suitable for this protocol). The experimental observations using a split-by-story splitting protocol on Huth's

dataset were in line with that achieved by using the split-by-stimuli protocol. Please refer to our code repository (https://github.com/YeZiyi1998/Brain-language-generation) for data partitioning options and all the experimental results on the Huth's dataset.

## B.2 Control model

Our study employs a generative modeling approach to reconstruct language from brain recordings, which differs from previously proposed approaches that involve a pre-construction and a classification step. This necessitates the design of control models to compare the approach to empirical lower-bound models. While it is possible to quantify accuracy like existing classification-based approaches to a certain degree, such as reporting a 65.8% probability of generating the next word from the vocabulary of 32,000 each time, this accuracy stems from a combination of brain input and the provided text prompt. Therefore, it is necessary to compare it with the control model based only on the text prompt to study and analyze the effect of brain input. The model based only on the text prompt employs only a standard LLM without external decoded input and thus quantifies the baseline performance of the LLM independently of the brain recordings input. It has been verified to be powerful in continuous language generation [5]. However, the LLM outputs are based solely on the knowledge learned from the training data crawled from the Web, which may not align with the individual's perception. Hence, we intend to examine the impact of brain input on language generation by comparing our proposed model to control models and probing whether brain input modeling can facilitate language generation that aligns more closely with the content perceived by human participants.

The first control model is a standard LLM which only has the text prompt input (StdLLM). In this comparison, the input of BrainLLM is the brain embedding, two special tokens for decoration the brain embedding, and the text prompt embedding. The input of StdLLM is only the text prompt embedding.

However, BrainLLM has more input tokens than StdLLM, and these tokens are either the output of a trainable brain adapter (brain embedding) or are themselves trainable tokens (special tokens). Hence, during the training process, the additional tokens in BrainLLM may encode information about the data distribution of token usage. This phenomenon, extensively studied in the context of prompt tuning [6–8], is effectively employed to generate language that mirrors the style observed in the training set. Although we have meticulously ensured that the stimuli in the training, validation, and test sets are entirely non-overlapping, they may still share a common data distribution of token usage due to their shared origin. For instance, all stimuli in Pereira's dataset adhere to a Wikipedia-style format and exhibit a token usage distribution akin to that of Wikipedia. Another way to interpret this effect is that even if the brain response is not sampled from the currently perceived continuation, it can still guide the language model to generate the language content that it is sampled from. This indicates that it may guide the LLM to generate content that is sampled from a single dataset and may exhibit similarities to the currently perceived continuation.

Therefore, the difference between BrainLLM and StdLLM may not only lie in the information about the currently perceived continuation that may be decoded from the brain but also in the effect brought by the information of token usage encoded in additional learnable tokens. In order to eliminate these effects, we permutated the brain inputs as additional baseline PerBrainLLM.Given a series of $n$ prediction tasks $\{B_i, W_i, M_i\}_{i=0}^{n}$ where $B_i$ is the brain responses corresponding to the text prompt $W_i$ and the content continuation $M_i$, we randomly shuffle the dependencies of brain responses and the text prompt for testing PerBrainLLM, i.e., $\{B_{k_i}, W_i, M_i\}_{i=0}^{n}$, where $\{k_i\}_{i=0}^{n}$ is a permutation of $\{0, ..., n\}$. In PerBrainLLM, the brain input does not necessarily correspond to the currently perceived continuation but may be sampled from participants' responses to any language content in the dataset. This allows us to study the impact of the semantic information about the currently perceived continuation contained in the brain while mitigating the effect of adding additional tokens. In this paper, we predominantly employed PerBrainLLM as the baseline across most of the analysis, as our primary focus lies in the effect of the information from brain recordings on the currently perceived continuation.

To further explain the difference between BrainLLM and its control models, we include a comparison of them from a probability perspective. As we have addressed in the Method section, in the generation task, the expected output is the perceived continuation $M = \{m_1, \ldots, m_k\}$, the input information is the brain

input $B$, and the text prompt input $W = \{w_1, \ldots, w_n\}$. Hence, the task can be simplified as estimating the generation likelihood of $M$ as $P(M \mid B, W)$. When no brain input is given, the generation likelihood of $M$ is $P_{LLM}(M|W) = q(M_{LLM} \mid W_{LLM})$, $q(M_{LLM} \mid W_{LLM})$ is the prior distribution of language generation in the standard LLM. When brain input is given, the generation likelihood with brain input is $P_{BrainLLM}(M \mid B, W)$, and its marginal probability is $P_{BrainLLM,M}(M \mid W) = \sum_b P(M_{dataset}, B = b \mid W_{dataset}) = q(M_{dataset} \mid W_{dataset})$, where $q(M_{dataset} \mid W_{dataset})$ is the distribution of language generation in the given dataset (textual stimuli). $q(M_{dataset} \mid W_{dataset})$ is different from $q(M_{LLM} \mid W_{LLM})$ as the text distribution is different in the given dataset and the dataset to train the standard LLM. Therefore, when $B$ is permuted as $\tilde{B}$ and may not provide information regarding the currently perceived continuation, we can assume that $\tilde{B}$ and $M$ are independent. Thus, the posterior probability is have the posterior probability of $P_{PerBrainLLM}(M \mid \tilde{B}, W)$ as follows:

$$
\begin{aligned}
P_{PerBrainLLM}(M \mid \tilde{B}, W) = \frac{P(\tilde{B}, W \mid M)P(M)}{P(\tilde{B}, W)} &= \frac{P(B)P(W \mid M)P(M)}{P(B, W)} \\
&\propto q(M_{\text{dataset}} \mid W_{\text{dataset}}) = P_{BrainLLM,M}(W \mid M)
\end{aligned}
\tag{1}
$$

This indicates that $P_{PerBrainLLM}(M \mid B^*, W)$ is in direct proportion to the marginal probability of $P_{BrainLLM}(M \mid W)$. Hence, the performance difference between BrainLLM and PerBrainLLM is solely due to the information gained from selecting brain samples corresponding to the perceived continuation, and is not related to the learned data distribution of token usage $q(M_{\text{dataset}} \mid W_{\text{dataset}})$ obtained during the training process.

## B.3 Exploring architectural variations of BrainLLM

To design BrainLLM's architecture, we explored a lot of structure variants and training objectives. The exploration encompassed the structure of the brain adapter, options between end-to-end training or prompt tuning, the effect of the warm-up step, and the possible integration of a contrastive learning target. This section elaborates on the experimental results of testing these variants in Huth's dataset (the dataset with the largest data size for each participant).

### B.3.1 Brain adapter structure

The brain adapter transforms the brain input as a time series $B = \{b_1, \ldots, b_t\} \in \mathbb{R}^{t \times c}$ into a series of embeddings $\{v_1^B, \ldots, v_t^B\} \in \mathbb{R}^{n \times d}$ which has the same shape as the text embeddings in the LLM. The structure is selected from a series of models, including Multi-layer perception (MLP) with position embeddings (see 14(a)) Recurrent Neural Network (RNN) (see 14(b)), MLP without position embeddings (see 14(c)), input concatenation with MLP (see 14(d)), and a linear model. We adopted hyperparameter selection for these variants. For the MLP, the number of layers was chosen from $\{1, 2, 4\}$, and the dimension of the hidden layers was selected from the set $\{500, 1000\}$. For the linear model, both first-order and second-order regularization terms were considered and selected from $\{0, 0.5\}$ and $\{0, 1.0\}$. For the RNN model, we considered the hidden layer dimension selected from the set $\{500, 1000\}$ and considered the structure variants of a standard RNN and an LSTM. Experimental results are presented in Table 18. Among the selection of variants, we find that MLP with position embeddings achieves the best win rate of 0.7893 of BrainLLM versus PerBrainLLM. The design of our brain adapter shares similarities with the work of some multimodal image-to-text models [9] and audio-to-text models [10–12], both aiming to map the representation of one modality onto another. Their studies found that a linear model could yield quite satisfactory results. However, our findings suggest that, in the context of a brain adapter, an MLP significantly outperforms a linear model. This implies that the brain's representations may not correlate as straightforwardly and effortlessly with natural language representations as image representations do, potentially requiring the advanced interactive capabilities afforded by an MLP versus a simpler linear model.

Another variant worth mentioning is that we set the output of the brain adapter as a series of embeddings $\{v_1^B, \ldots, v_t^B\} \in \mathbb{R}^{n\times d}$, with the same length $t$ of the brain input. We also consider a variant of the output $\{v_1^B, \ldots, v_{t'}^B\} \in \mathbb{R}^{n\times d}$ in which $t$ is not necessarily equal to $t$. We test these variants based on Multi-layer perception (MLP) with position embeddings. For any $t'$, we set the dimension of the output of the MLP layer as $d \cdot t'/t$, where $d$ is the dimension of the token embeddings in the LLM. Then the output of the MLP layer can be decomposed or concatenated into $\{v_1^B, \ldots, v_{t'}^B\} \in \mathbb{R}^{n\times d}$ with each $v_i^B$ has the dimension of $d$. We test $t'$ selected from $\{1, t/2, t, 2t, 4t\}$ and find $t' \in \{t, 2t\}$ archives best performance in Huth's dataset, with their differences being statistically insignificant. Therefore, for simplicity, we opted to select $t' = t$.

### B.3.2 Prompt tuning v.s. fine-tuning

We implemented a prompt-tuning protocol to train BrainLLM, which frozen the LLM's parameters while training only the brain adapter and specific tokens using gradients derived from the LLM. Additionally, fine-tuning with full parameters is a common alternative, although it use higher computational costs due to the vast number of parameters requiring tuning. Numerous studies have been conducted to compare these two methods, and the general conclusion is that fine-tuning yields slightly better results for specialized tasks that do not require strong generalization ability. On the other hand, prompt tuning has lower training costs and potential for better generalization. The improved generalization ability associated with prompt tuning becomes increasingly significant with the increase of the model's parameter size.

Considering the costs associated with full parameter fine-tuning on the Llama-2 model, we carried out experiments comparing full parameter fine-tuning with prompt tuning on the GPT2-xl. Given that the learning rate requirements for full fine-tuning is usually different from prompt tuning, we conducted fine-tuning experiments across a wide range of learning rates, from $1 \times 10^{-3}$ to $1 \times 10^{-7}$. We then presented the best results for direct comparison with the results of prompt tuning. In addition, we tested a combined strategy by initiating full parameter fine-tuning based on the checkpoint of prompt tuning, with learning rates also selected from $1 \times 10^{-3}$ to $1 \times 10^{-7}$. The experimental results are presented in Table 19. From Table 19, we observe that full parameter fine-tuning yields worse performance than prompt-tuning. This observation contradicts findings in connecting other modalities with LLMs [9–12]. One potential explanation for the weak performance could be the incomplete training of the newly introduced brain adapter and special tokens. In contrast, the original generative capabilities of the LLM may be hurt in the training. Actually, we observed that the loss on the validation set becomes stable at a relatively high level during training, while the training set exhibited overfitting with low training loss at the same time. Then, we tested the combined strategy and found it outperforms the full parameter fine-tuning strategy. However, this did not enhance the performance achieved by prompt tuning. In our experiment, we find the optimal learning rate of the full parameter fine-tuning combined strategy was $1 \times 10^{-7}$, with the results reported in the table. Moreover, we observed an increased performance of the combined strategy with the smaller learning rates, indicating the stage of full parameter fine-tuning might not be beneficial. Notably, with even smaller learning rates—though typically not used for LLM fine-tuning ($<1 \times 10^{-8}$), the combined strategy still underperforms prompt tuning.

### B.3.3 Effect of warm-up step

The warm-up step is designed to prevent the outputs of the brain adapter from being entirely different from to the LLM's language embedding space during the initial stage of training. If a warm-up step is not applied, the training stage will lead to gradient explosion, which, although mitigable by gradient clipping, may affect the stability during training and introduce additional hyper-parameters. We conducted experiments without warm-up stage on three datasets. The win rates of BrainLLM versus PerBrainLLM on the Huth's, Pereira's, and Narratives datasets are 62.1%, 78.7%, and 64.1%, respectively. We observed that warm-up stage did not significantly improve performance on the Huth's dataset but did significantly enhance performance on the other two datasets.

### B.3.4 Discussion on loss function

During training, we adopted a cross-entropy loss function based on next token prediction, the same as the loss function used in training LLMs for natural language processing. Recently, contrastive learning loss functions have become popular; however, they seem challenging to adapt it into our framework. One potential approach is to align brain embeddings with the embeddings calculated by the text preceding the text prompt (referred to as the pre-text prompt). This approach can help the brain adapter to learn a representation that can convey similar information of pre-text prompt content and facilitate the generation of the perceived continuation. However, simply using the pre-text prompt to construct contrastive learning pairs does not guarantee an increased likelihood of generating the perceived continuation, and thus this optimization may not directly improve the final objective. Our experimental results showed that incorporating this loss did not enhance performance; for instance, on the Huth dataset, a loss weighting of 0.1 resulted in an average win rate of 74.3%. Future work may need to investigate whether to introduce new loss functions when incorporating brain recordings into the joint training with LLMs, or solely focus on token generation loss as in traditional language model training.

## B.4 Extended Reuslts and Discussions on Measurements

This section presents extended reuslts and discussions on measurements to investigate BrainLLM and its baselines and controls, including *relationship bwteeen the length of the text prompt and the win rate*, *language similarity metrics without function words*, and *relationship between the measurements*.

### B.4.1 Relationship bwteeen the length of the text prompt and the win rate

In the results section, we show that there is a negative correlation between the length of the text prompt and the win rate. We further conduct an analysis based on structural equation modeling (SEM) to investigate the effect of context length on the decoding performance of Pereira's dataset. The dependent variable is the win rate while the independent variable is the context length. The effect of context length can be associated with a series of mediator variables, including the surprise level, the different mechanisms between the brain and LLMs [13], and so on. As a preliminary experiment, we only use the surprise level as a mediator variable, as other factors are difficult to quantify and control. The analysis yielded a coefficient of 0.041 for the surprise level (effect of the mediator on the dependent variable) and 0.005 for the context length (direct effect of the independent variable on the dependent variable), with significance level $p = 9e^{-14}$ and $p = 0.004$, respectively. This indicates that surprise level plays a major role in the SEM analysis. However, as there still exists a direct effect related to context length, other factors, including the different mechanisms between the brain and LLMs, may also exist.

### B.4.2 Language similarity metrics without function words

As the qualitative results may be biased due to function words, we also conducted an additional experiment to compare the similarity scores of both BrainLLM and Tang et al.'s methods. Specifically, we calculate the language similarity metrics on the reference content and decoded content after filtering the function words with the NLTK stopwords library [1]. Experimental results are presented in Table 12 (full-text reconstruction) and Table 22 (language continuation generation). We observe that, after the filtering, there is a notable performance gap between the full-text construction and the language generation task which predicts a continuation based on a text prompt. This implies that the accuracy of the full-text reconstruction task is significantly lower than that of the proposed language generation task. However, in both task settings, BrainLLM outperforms Tang's method and the baseline where randomized brain signals are used as input (PerBrainLLM).

Despite the superior performance of BrainLLM, open-vocabulary decoding for full-text reconstruction remains highly challenging at a level that could immediately lead to practical applications. For this reason,

[1] https://www.nltk.org/

to obtain more comprehensive and fair evaluation results, we also investigate reconstruction results with two alternative setups. (1) evaluate language reconstruction performance on the proposed language generation task which predicts a continuation based on a text prompt; (2) conducting more comprehensive evaluation and comparison with multiple metrics: for example, language similarity metrics with or without function words and the comparisons of the likelihood on generating the ground truth content.

### B.4.3 Relationship between the measurements

Our statistical analyses show that BrainLLM is significantly better than PerBrainLLM across the three metrics of win rate, language similarity metrics, and human evaluation. Those metrics are based on different perspectives and have both connections and differences. This section provides a more fine-grained analysis of them.

First, all measurements are positively correlated with each other, indicating that these evaluation methods have some shared objectives for accurate semantic decoding. For win rates and human preference, we observe that when BrainLLM is preferred over PerBrainLLM, the average win rate is 80.8%. When BrainLLM draws with PerBrainLLM, the win rate is 74.1%. Conversely, when BrainLLM is not preferred to PerBrainLLM, the win rate is 66.7%. This indicates that higher human preferences correlate with better metric scores in terms of win rates. For win rates and language similarity metrics, we investigate experimental results in Huth's dataset and show that The language similarity metrics for the winning samples are significantly better than the loss samples, including higher metrics for the winning samples in BLEU-1 ($Mean_{diff} = 0.035, p = 9.9e^{-38}$, one-sided paired t-test), ROUGE-1 ($Mean_{diff} = 0.034, p = 5.7e^{-37}$, one-sided paired t-test), and ROUGE-L ($Mean_{diff} = 0.035, p = 1.4e^{-37}$, one-sided paired t-test), and lower metrics for the winning samples in WER ($Mean_{diff} = -0.0029, p = 2.4e^{-31}$, one-sided paired t-test). For the relationship between a series of language similarity metrics and human preference, we present an analysis in Fig. 17. As shown in Fig. 17, human preference between BrainLLM and PerBrainLLM is generally associated with higher language similarity metrics. For example, when BrainLLM is not preferred to PerBrainLLM, its word error rate is 0.16% higher than that of PerBrainLLM. In contrast, in cases where BrainLLM is preferred, the word error rate is 2.69% lower, indicating that the predicted content from BrainLLM is more accurate than that from PerBrainLLM.

Second, among these metrics, the win rate based on surprise (or perplexity) directly accesses the generation likelihood of ground truth content, which is a newly used metric for language decoding with brain input but has been commonly used in language modeling tasks. A win rate above 50% indicates that BrainLLM has a higher likelihood to generate the ground truth content versus PerBrainLLM. On the other hand, human evaluation and language similarity metrics are based on comparing the actual content generated by BrainLLM and PerBrainLLM. Given the variety of language space, a higher likelihood of generating the ground truth content does not necessarily indicate that the actually generated content is better. Here we provide several examples in Table 23. In the first and second cases, BrainLLM wins PerBrainLLM. However, in the first case, BrainLLM generates the same content as PerBrainLLM, leading to a draw in human evaluation. In the second case, PerBrainLLM generates more terms aligned with the perceived continuation and is preferred by human annotators, even though its likelihood of generating the perceived continuation is lower than BrainLLM. This phenomenon occurs because in many cases, a model with a lower likelihood of generating ground truth can perform better simply because it coincidentally generated relevant semantic content from the vast language decoding space. Therefore, this statistical analysis between win rate and human evaluation demonstrates that a higher generation likelihood correlates with better actually generated content, even though they do not always align.

Third, although both language similarity metrics and human evaluation are based on the actually generated content, there may be discrepancies between them in some cases. For example, the third case in Table 23 presents a sample in which BrainLLM and PerBrainLLM have the same language similarity metrics, but BrainLLM's output is actually more semantically accurate. In the fourth case, PerBrainLLM's output has a higher language similarity score and wins in terms of surprise, but humans may prefer BrainLLM outputs because "realize" and "make sure we all got" have similar meanings. Language similarity metrics are more

objective and reproducible, but as shown in the example above, they might fail to capture semantic content beyond accurate matching. Therefore, we combine the above three measurements to evaluate BrainLLM more comprehensively.

### B.5 The pre-construction followed by post-hoc selection approach [14]

Tang *et al.* [14] propose a pre-construction followed by post-hoc selection approach to reconstruct continuous language from BOLD signals. They used a standard GPT model and an encoder as independent post-hoc models for language reconstruction. Building upon the publicly available GPT (or GPT-1) model [15], they further refined its capabilities by fine-tuning it on a corpus encompassing Reddit comments (exceeding 200 million words in total) and 240 autobiographical narratives from The Moth Radio Hour and Modern Love. A brain encoder is trained to estimate a set of weights that quantify the impact of the perceived continuation (represented by GPT embeddings) on the BOLD signal in each voxel. With the GPT model and the brain encoder, they reconstruct the language with the following process. First, the GPT model is used to pre-generate the top-ranked next tokens with a threshold probability when given the text prompt. This pre-construction process incrementally builds up a sequence of tokens as the continuation of the given text prompt. Using a beam search algorithm with a width of 200, the continuation candidates can be pre-generated with the GPT model. Second, to avoid exponential combinations during the generation process, the model accepts a maximum of five continuations for each candidate by measuring how well the recorded brain responses match the brain responses predicted by the pre-generated candidates. The pre-generation step is used with a restricted subset of 6,867 tokens to tackle the challenge of generating text with a vast vocabulary. The generated outputs from their approach are then compared to those from a standard LLM (i.e., GPT in their paper) in terms of language similarity metrics.

Different from our experiments, Tang *et al.* [14] did not test and analyze the model performance regarding text prompts with varying lengths. They based their approach on several pre-defined initials consisting of only one token (e.g., "I", "He") as text prompts, followed by continuous generation based on content that has been previously generated. These initials provide limited information and may not necessarily be the same as the actual text prompts. Hence, their setting is more similar to the setting of language generation without any text prompts in our experimental setup, which also provides a few text prompts for language generation. On the other hand, the token combination of the perceived continuation may not be within the beam search width during the beam search process used in their approach. As illustrated in their article, their model is typically unable to generate content that is entirely identical to the perceived continuation. This also implies that their model can not estimate the generation probabilities of the perceived continuation, as the sequences including the perceived continuation are often pruned during the beam search process. As a result, they could not use win rate as a metric for evaluation in the same way as we do in our evaluation, but only used a language similarity metric.

To make a fair comparison between Tang *et al.* [14]'s model and ours, we reproduce their model with the same configurations for the LLM selection, token vocabulary, evaluation dataset construction, and metrics as ours. The differences between our reproducibility and their original proposed approach are listed below: Firstly, instead of using a private GPT model, the PerBrainLLM based on a publicly available Llama-2 is used for pre-generating candidates. No restriction is applied to the size of the vocabulary (they use a restricted vocabulary), and thus the whole token vocabulary of 32,000 is adopted in the generation process. Using PerBrainLLM for pre-generating candidates means that the method reproduced in our experiments may have a stronger performance than the originally proposed method. Secondly, instead of generating from some pre-defined initial tokens, generation with and without the actual text prompts are both adopted in our comparison for analysis. Thirdly, their model calculates the language similarity metric over the entire text content perceived by the participant during an fMRI recording, approximately 16,400 tokens. This means that, as their paper states, the content generated at any time frame may have shared similar tokens with the perceived content in the other time frame, thus leading to higher language similarity metrics. We, on the other hand, only consider the current time frame in which participants usually perceived about 3-10 tokens, and use the generation output with corresponding brain recordings to calculate the language similarity metrics.

This makes the results more targeted, even though they may appear lower on the metric. Finally, due to the infeasibility of estimating the generation probabilities of perceived continuation, only the language similarity metrics (i.e., BLEU-1, ROUGE-1, ROUGE-L, and WER) are used in comparisons involving their models.

LLMs inherently possess the capability to generate the next token. Our method builds on this capability and employs a brain adapter to transform brain inputs to directly influence the computation and generation of LLMs. This comparison demonstrates that the generation of LLMs is more aligned with the participant's perceived semantics when incorporating brain signals. While Tang's method appears to achieve similar objectives to ours, in addition to significant differences in methodology, there are also some key differences in terms of their effectiveness and application scenarios. First, we demonstrate that our method is more effective in both language continuation generation and full-text reconstruction tasks. This is because our approach transformed brain representations as inputs for language models, which is motivated by evidence suggesting a connection between brain signals and LLM representations [16–19]. In addition, our method can also address cases in which LLMs fail to include the correct candidates among the top candidates for selection. Second, since our method does not require candidate generation and post-selection, it can directly estimate the generation probability of any text continuation. Therefore, we also propose analyses based on win rate and surprise level. Such analyses can lead to more applications; for example, neuroscientists can use BrainLLM to estimate the likelihood of any semantic content encoded in the human brain rather than a small set of semantic candidates. This may extend existing paradigms for studying the representation and formation of language in the brain. Third, Tang's method is influenced by the Bayesian-based statistical language modeling in early NLP research, whereas the current mainstream trend favors building end-to-end generative models. BrainLLM utilizes a generative method which has been considered to have scaling capabilities and better adaptability in the field of generative AI. For example, we also conduct analyses related to scaling the data size and the parameter size of generative AI models. This provides significant insights for combining generative AI with neurophysiological data.

## B.6 Discussions on full-text reconstruction

The full-text reconstruction experiment is conducted following the evaluation setup used in Tang *et al.* [14]'s work, which involves reconstructing the content of an auditory stimulus story named "Where There's Smoke" of approximately 10 minutes in length. The experiment is conducted by testing the full-text reconstruction performance of the proposed model BrainLLM and its control PerBrainLLM with permutated brain inputs and a null model without brain input (StdLLM). We also presented the performance of Tang *et al.* [14] as well as its null model's performance (which uses a private LLM backbone). Additionally, we re-implement the Tang *et al.* [14] with permutated brain inputs. We use the same evaluation method as Tang *et al.* [14]. The metrics are calculated based on the predicted and reference words within a 20-s window around every second of the stimulus (window similarity). The scores were then averaged across windows to quantify how well the decoder predicted stimulus.

Experimental results are presented in Table 25. From Table 25, we observe that in terms of the null model's performance, Tang *et al.* [14] outperforms BrainLLM. Tang *et al.* [14] uses a private language model that is trained in a corpus constructed with Reddit stories, which is similar to the perceived story content. On the other hand, we use a publicly available language model GPT2-xl which is trained in a general corpus and therefore shows worse performance when compared to Tang *et al.* [14] when no brain input is given. However, we observe that the proposed BrainLLM shows comparable performance with Tang *et al.* [14]'s method in all language similarity metrics with brain inputs. A pair-wise t-test shows significant improvements are only observed in METEOR ($p = 3e^{-5}$), and in WER ($p = 0.03$). We also test a more fair control with the brain input permutated. The experimental results demonstrate that our method significantly outperforms PerBrainLLM in metrics of BLEU-1 ($p = 3e^{-4}$), and WER ($p=5e^{-4}$). Additionally, we tested Tang *et al.* [14] with permutated brain inputs, it outperforms the null model based on the BLEU and METEOR metrics. The reason could be that the classifier trained for post-hoc selection tends to select content that is stylistically similar to the training data, which potentially contributed to the superior performance of the permutated model compared to the null model.

However, full-text reconstruction is challenging, we recognize that both BrainLLM and Tang *et al.* [14]'s approaches perform far from perfect matching in this task. Often, the successfully matched words are function words or stop words, which limits the significance of the outcomes (see Table 16). Moreover, there is a noticeable performance gap compared to the proposed language generation task (in comparison with Table 4). Although quantitative metrics are used to evaluate the performance of full-text reconstruction, these assessments are significantly influenced by the language styles produced by different base LLMs. Therefore, the practical usefulness of language decoding models for full-text reconstruction requires further testing. We believe that full-text reconstruction using brain signals necessitates sustained investment, encompassing not only software algorithms but also more accurate BCI devices. However, in the current stage, the language generation task we provide may offer an alternative possibility—combining this method with motor-based BCI through collaborative work to achieve more efficient generation. For instance, our method could generate a set of candidates, which are then selected and confirmed using motor-based BCIs.

## B.7 Summary of recent effort on neural language decoding with LLMs

Decoding natural language from brain signals remains a significant challenge and has typically been achieved in a classification setup by selecting from a corpus of pre-defined words or sentences. Recently, semantic decoding with the help of LLMs is a rapidly emerging field of research. The ability of LLMs to generate continuous language makes it possible to decode non-predefined semantic content. Tang *et al.* [14] propose a pioneering research in which LLMs are applied to generate a corpus of semantic candidates while brain signals are applied in a post-hoc selection phase to select the most likely content. BrainLLM removes the traditional selection-based paradigm by directly using brain signals as input to the large language model for direct generation.

While during the period of constructing and testing BrainLLM, we noticed a considerable amount of related work. According to the validation method, the research could be categorized into three groups: (i) full text construction (FTC), (ii) teacher forcing (TF), and (iii) text continuation (TC). Full text construction (FTC) means the decoder needs to construct full text with only brain signals, which can be up to a passage or a story. Teacher forcing (TF) means the decoder can predict the next token by using the actual target output as the next input, rather than using the output predicted by the decoder itself. Text continuation (TC) means the decoder constructs a text continuation based on existing semantic contexts. TF is criticized by Jo *et al.* [20], as providing the target as input leads to good decoding performance, so it should be evaluated more strictly. Different from TF, TC and FTC can not use the actual target output, which makes the results more comprehensive. One of the differences between TC and FTC is that there is still a significant gap between the performance of TFC and its practical usability. In contrast, TC achieves practical usability but requires the decoder to access additional user-related context information, such as what others have said to this user, to use as a text prompt.

Here we summarize a series of existing research in different groups in Table 10, with their performance on different datasets. Under the TF setting, Wang *et al.* [21] and Xi *et al.* [22] map EEG and fMRI features to the embedding space of a transformer-based sequence-to-sequence model BART. Dewave [10] further proposes to utilize discrete encoding for the representation of EEG features. Under the FTC setting, NeuSpeech [23] treats neural decoding as a speech-decoding task and aligns MEG recordings with Whisper representations to accomplish open-vocabulary full-text reconstruction. MAPGuide [24] proposes a two-stage approach similar to Tang *et al.* [14]'s but directly selects the text continuation by comparing them with the predicted text embeddings mapped from brain activities. PREDFT [25] build upon BrainLLM and propose a side network that utilize the theory of predictive coding to improve the decoding performance. BP-GPT [26] is the work most similar to ours from the same period, also utilizing the adapter method for decoding. However, there are significant differences in their robustness design, word rate model design, and experimental design, which we further discussed in Section B.7.1.

Note that their performance can not be compared directly as they use different validation protocols and datasets. However, we can conclude several trends according to Table 10. First, TF is less commonly adopted in more recent research due to its improper settings. Second, different signals may have varying decoding

capabilities. Notably, there is no research in this table showing that EEG can be used to decode language under the setting of TC or FTC, while MEG and fMRI have been shown to be effective under the setting of TC or FTC. Third, generative approaches that combine brain representations as input into language models are gaining popularity over methods using brain representations in a post-hoc phase (MAPGuide and Tang et al.). Finally, the decoding performance can vary across datasets with different types of stimuli, possibly because LLMs themselves exhibit varying perplexity with different language contents.

### B.7.1 Comparison with BP-GPT

Among these research, the most related work is BP-GPT [26]. We noticed that this paper was first published on May 13, 2024 (arxiv version), while our first version was published on November 16, 2023 (arxiv version). That means the two were probably contemporaneous works. Here we compare the performance of BP-GPT, Tang et al.'s method, and BrainLLM in Table 15. As shown in the table, both BrainLLM and BP-GPT are comparable to or outperform the method proposed by Tang et al., indicating the superiority of a generative setup. We observe that Tang et al.'s method shows comparable performance with BP-GPT and BrainLLM in terms of BLEU-1. Tang et al.'s method's strong BLEU-1 performance may be attributed to its private GPT-2 which was pre-trained on a corpus whose token usage is similar to the stimuli's style. However, when measured by METEOR, which considers both the token-level accuracy and their orders, it exhibits significantly lower performance. When comparing BP-GPT and BrainLLM, we observe that BrainLLM with GPT-2-xl outperforms BP-GPT in terms of BLEU-1 and METEOR for most subjects, except for METEOR for subject 1. When using the GPT-2 model of the same size, BrainLLM and BP-GPT exhibit more similar performance.

Given their distinct innovative design concepts and methods, comparison only based on the numerical results is not particularly meaningful. Here we list the three key differences regarding the novel designs between BP-GPT and the proposed BrainLLM. First, BP-GPT uses an external text-to-text baseline to align the fMRI prompt with the text prompt, which helps extract a more robust brain prompt. BrainLLM also incorporates designs for robustness. However, BrainLLM does not introduce external information while using a specially designed brain adapter architecture and the implementation of a warm-up loss to deal with the noisy fMRI data. Second, BP-GPT uses a special token to segment text based on the repetition time (TR) of fMRI while BrainLLM uses a word rate model followed by Tang et al. The experiments on BP-GPT show that using special tokens outperforms a word rate model, although additional training for GPT2 is required. BrainLLM does not contribute to the word rate model but rather to exploring variants of different adapter structures and training methods for the decoding model. Third, BP-GPT conducts experiments with GPT2 (fine-tuned or no fine-tuned) and on three subjects on Huth's datasets. As a technical paper for computer science audiences, they devoted more sections to explaining the design of each technical module and the ablation study. BrainLLM conducts more experiments on different sizes of LLMs, datasets consisting of different stimuli, and more participants. BrainLLM also conducts in-depth analysis regarding the surprise levels, the text prompt, the size of datasets and LLMs, and the ROIs. These analyses help general audients better understand how the brain decoding technology evolved in the era of LLMs across different language contexts, varying sizes of machine models, and decoding content of different difficulty levels.

## B.8 Ethical issues

The development of BCI technology to reconstruct language from the human brain raised significant concerns about privacy and informed consent. The capability to directly access and decode brain signals could facilitate covert monitoring of individuals' thoughts, challenging the deeply ingrained notion of the mind as a private sanctuary, solely accessible to its owner. While this technology has the potential to revolutionize communication, self-expression, and mutual understanding, it also raises concerns about privacy, manipulation, and the very essence of free will [27]. Although such technology is currently at a very early stage where such applications feel a long way off, several existing studies have already discussed the associated concerns [14, 27, 28]. For example, Mecacci [28] developed several criteria to measure the ethical issue. Tang *et al.* [14]

observe that participant cooperation is required for language BCIs, which indicates that participants can consciously resist the language decoding process.

Nevertheless, existing language decoding methods follow a pre-definition [1, 29] or pre-generation step [14] to construct semantic candidates within limited topics before incorporating brain recordings to identify the most likely candidate from the pool. As the semantic candidate's pool could be safe and controllable under human heuristics, thoughts that may involve personal information can be precluded from the pre-definition or pre-generation step. However, this control is only effective if the pre-selection process is not subject to malicious attacks. It is still possible for illegal usage such as semantic decoding that may involve sensitive candidates. On the other hand, the proposed direct language generation approach does not have a human-controllable pre-definition or pre-generation stage. This implies that the entire generation process is completely motivated by the representations in the participants' brains and the LLM. Furthermore, the reconstructed language could be anything that is reflected in the brain responses. These features empower our model with greater freedom to generate personalized content compared to previous methods, but they also introduce the potential for decoding content that participants may wish to keep private.

We believe that the following aspects can be considered to mitigate this concern. Firstly, it may be necessary to avoid the generation of private content from the machine model's perspective. Considering the inherent complexity and lack of explainability of the LLM and the human brain, an applicable approach at this stage involves processing the output content with hand-crafted rules [30]. Secondly, rather than relying solely on post-hoc filtering for privacy information, we suggest preventing the model from accessing privacy content in the first place by designing and training a safe brain adapter. This approach can be accomplished by machine learning techniques such as feature selection and can ensure the model only generates task-relevant and non-private semantic information in the human brain. Finally, before it is fully ensured that the model will not output private content, the output should be reviewed by the participants. This review process may merely involve the participants deciding whether or not to share such content, thus requiring minimal user effort.

## B.9 Differences of Large language model (LLM)

BrainLLM adopts the GPT-2 series and the Llama-2 as backbone LLMs in its variants. The main differences between the GPT-2 and the Llama-2 are in their architecture, training data, and training process. (1) In terms of architecture, both models are composed of stacked transformers, but the number of layers and the dimensions of the hidden layers are different, which leads to different sizes of total parameters (see Table 17). Besides, the selection of normalization layers and activation functions, which are adopted for connecting the stacked transform layers, differs between the GPT-2 and the Llama-2 [5]. (2) They are also different in the construction of training data. The training data of the GPT-2 series were 8 million web pages and a total of 40 GB of text crawled by OpenAI [2], while Llama-2 is trained on 2 trillion tokens of text data collected by Meta [3]. (3) The training process of the GPT-2 series is entirely unsupervised, focusing solely on the task of predicting the next token. In contrast, the training regimen for the Llama-2 model is more multifaceted. It not only involves the unsupervised next token prediction task but also incorporates several supervised fine-tuning tasks, as well as reward modeling based on human feedback. This implies that Llama-2 not only learns the knowledge of generating continuous language from a large text corpus but also undergoes model correction to some extent through supervised knowledge and feedback involving human participation. Due to its large parameter size, efficient training data, and human involvement in tuning, Llama-2 is currently the strongest open-source model on many benchmarks, and it has comparable capabilities to several commercial-licensed language models [5].

## B.10 Discussions on Hyper-parameters

In our experiments, the learning rate is selected from $\{1 \times 10^{-3}, 1 \times 10^{-4}, 1 \times 10^{-5}, 1 \times 10^{-6}\}$ based on the experimental performance on Huth's dataset's validation set. These parameters were then directly applied

[2] https://openai.com/
[3] https://about.meta.com/

to Huth's dataset's test set and other datasets without additional hyperparameter tuning to ensure consistency and prevent potential overfitting. The experimental results in terms of win rates on Huth's dataset with different learning rate selections are shown in Table 21. We observe that a learning rate of $1 \times 10^{-4}$ yields the most optimal results, and it was thus selected for our experiments on other datasets and further analysis. Furthermore, given the inherent high dimensionality of fMRI data, we employed Principal Component Analysis (PCA) to reduce the dimensionality of fMRI data into a dimension of $c$. We select $c$ from $\{500, 1000, 2000, 4000\}$. We observe that both $c = 1,000$ and $c = 2,000$ dimensions yield optimal results, with no significant differences in performance. To balance between computational efficiency and model performance, we selected $c = 1,000$. Compared to existing methods (e.g., [1, 14]) that required consideration of a lot of hyperparameters such as regularization weights and the number of voxel selection, BrainLLM employs fewer hyper-parameters. This is primarily because BrainLLM leverages publicly available LLMs, thereby negating the need for further adjustments to the LLM's hyper-parameters.

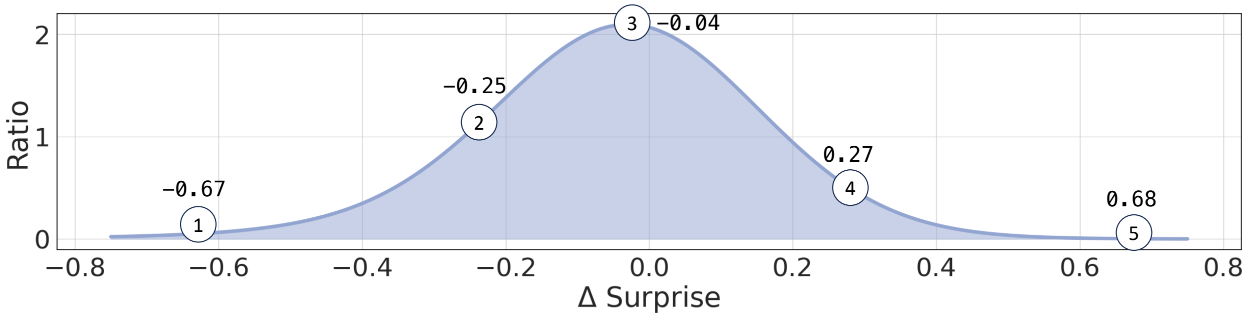


| | Text prompt | Continuation | BrainLLM prediction | Control prediction |
|---|---|---|---|---|
| 1 | They recorded if they recalled | any dreams, and described each | the dream, and if so, what it was about | the information later |
| 2 | Farms usually have a | house for farmers, a | house for the farmer and his or her family. | fence around them to keep livestock in and predators |
| 3 | An igloo is a type of shelter made from | blocks of snow by Inuit | blocks of snow | blocks of snow and ice |
| 4 | Sweaters are often | knitted from wool but | made of wool, cotton or synthetic fibers | made of wool, cotton or synthetic fibers |
| 5 | A painter must keep | many elements in mind | his or her brushes and paints clean to avoid | their brushes and paints clean to avoid |

**Fig. 1**: **Case analysis for Pereira's dataset.** The cases are randomly sampled based on the differences in surprise levels measured by BrainLLM and PerBrainLLM. A smaller surprise difference indicates that BrainLLM outperforms PerBrainLLM to a greater extent.

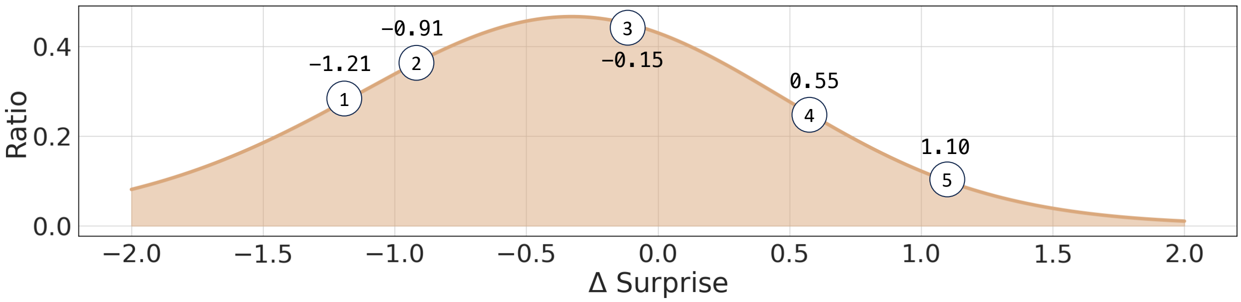


| | Text prompt | Continuation | BrainLLM prediction | Control prediction |
|---|---|---|---|---|
| 1 | looked at or thought about for | a couple months it like immediately goes to goodwill | a long time and i'm like | a very long time and it's my high school yearbook |
| 2 | what insurance companies | need use to know | don't want you to know | don't do is they don't tell you |
| 3 | and it's late spring and i go visit some | friends at princeton and yet again i get | friends in new york city and i'm staying with | of my cousins and they're all like oh my god it's so grea |
| 4 | force one a and the moral was | always the same any moment could be the | don't get your hopes up the white house is a big place and | always the same you never know when it's going to be your last |
| 5 | a few weeks into the job | the company got a really | i'm sitting in the oval office | i found myself in a meeting with the ceo |

**Fig. 2**: **Case analysis for Huth's dataset.** The cases are randomly sampled based on the differences in surprise levels measured by BrainLLM and PerBrainLLM. A smaller surprise difference indicates that BrainLLM outperforms PerBrainLLM to a greater extent.

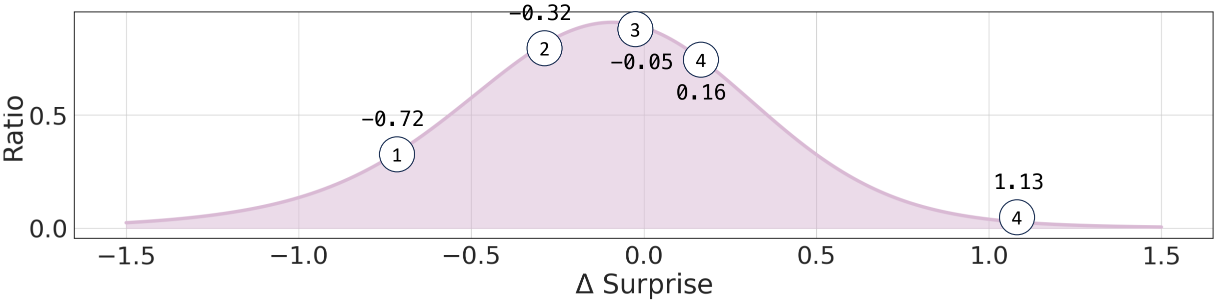


| | Text prompt | Continuation | BrainLLM prediction | Control prediction |
|---|---|---|---|---|
| 1 | we were just talking | about how you always | about this the other day uh and you said | one day and i said hey you know what's |
| 2 | she was like petite i could have | folded her up and put her my pocket she looked | picked her up with one hand and put her in the trunk of my car | put her in the trunk of my car and driven her to work every day |
| 3 | work for the new York times and i was working a story one time about mone | laundering on a little | laundering in the cayman islands and i was talking | aundering in the cay- man islands and so i went |
| 4 | walked out of a marriage or something or | is an alcoholic or both | a relationship or something like that um and so he's | a relationship or something like that and um he's kind |
| 5 | there's this girl in the | window um that i | hallway and she's kind of screaming | hallway and she‘s kind of looking at um |

**Fig. 3**: **Case analysis for Narratives dataset.** The cases are randomly sampled based on the differences in surprise levels measured by BrainLLM and PerBrainLLM. A smaller surprise difference indicates that BrainLLM outperforms PerBrainLLM to a greater extent.

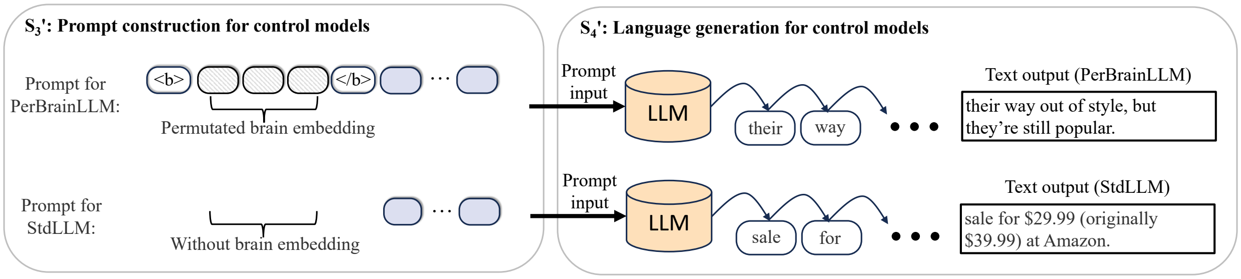


**Fig. 4**: **The schematic diagram for language generation with permuted brain recordings (PerBrainLLM) and without brain recordings (StdLLM).** $S_3$**'.** The prompt input for PerBrainLLM adopts a permutation of the correspondence between the sample of brain recordings and the perceived continuation. The prompt input for StdLLM is only the text prompt embedding, which acts as a standard LLM and generates the most likely continuations based on its training on internet-based data. $S_4$**'.** The content generated by PerBrainLLM and StdLLM maintains coherence with the text prompt but fails to align semantically with the perceived continuation.

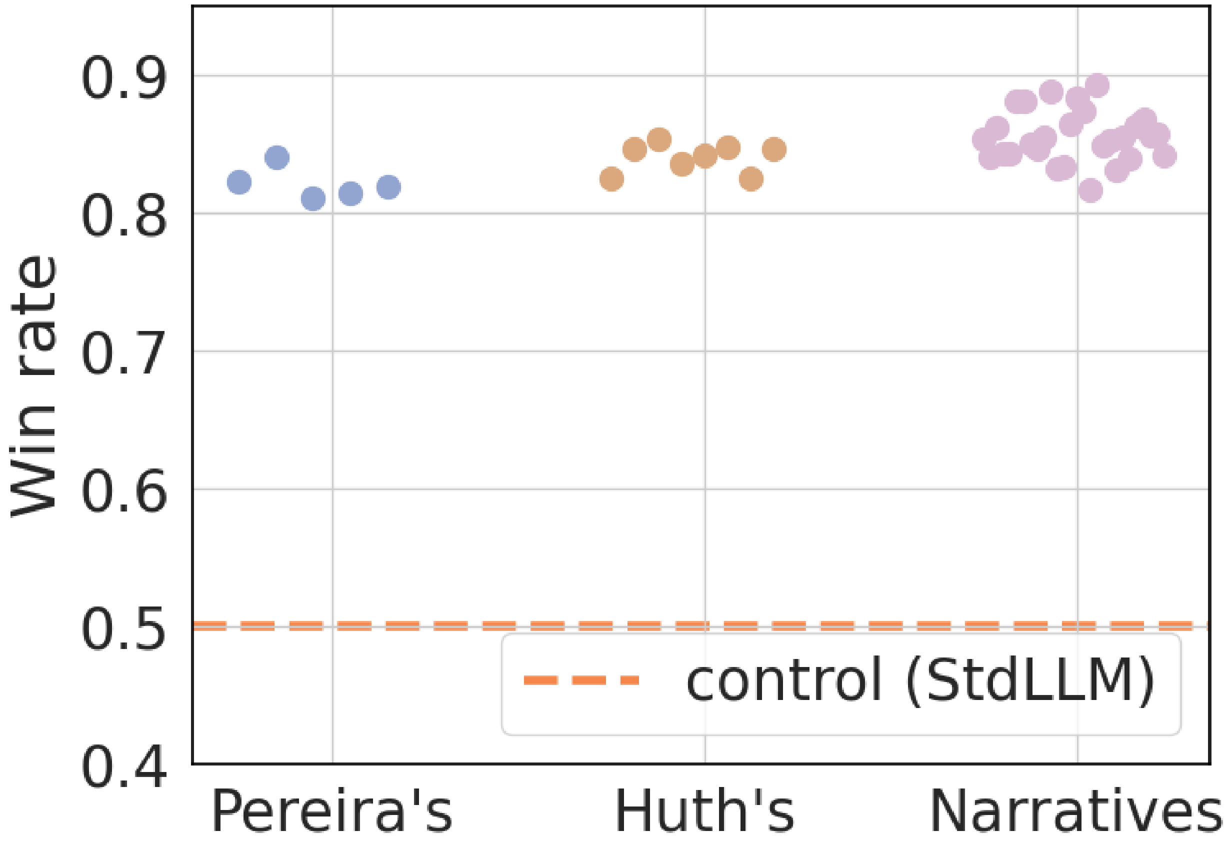


**Fig. 5**: **Win rate of BrainLLM vs. StdLLM.** Each dot represents the win rate of a single participant in Pereira's dataset (5 participants), Huth's dataset (8 participants), and Narratives dataset (28 participants).

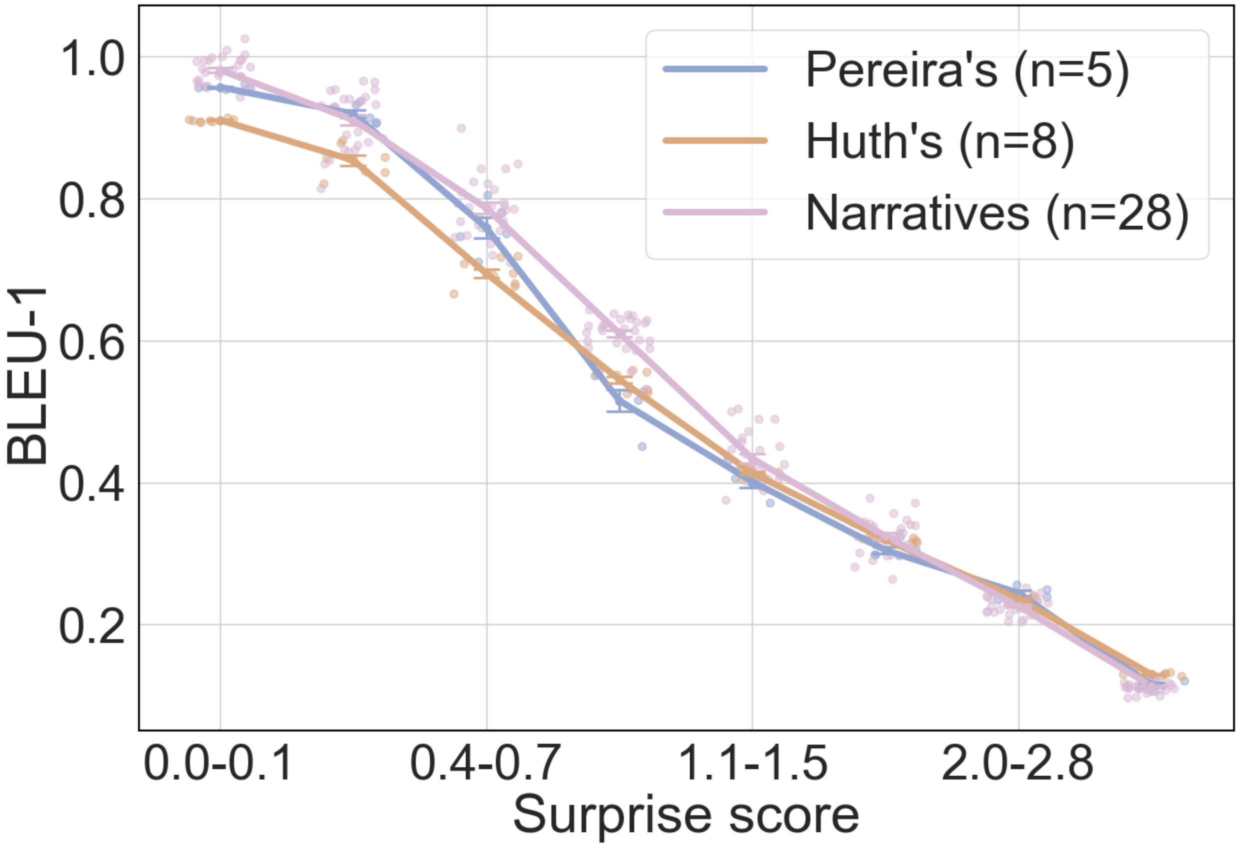


**Fig. 6**: **BLEU-1 score of BrainLLM across perceived continuation with different surprise levels.** The Pearson's coefficient $r$ between the surprise levels and the BLEU-1 score in Pereira's dataset, Huth's dataset and Narratives dataset are -0.66, -0.52, and -0.56, respectively. This observation suggests that with an increased surprise level, it becomes more difficult for the LLM to generate the perceived continuations. However, the negativity of this coefficient is smaller than that of PerBrainLLM, indicating that as the surprise level increases, the performance of BrainLLM decreases less than that of PerBrainLLM. Error bars denote mean +/- SEM.

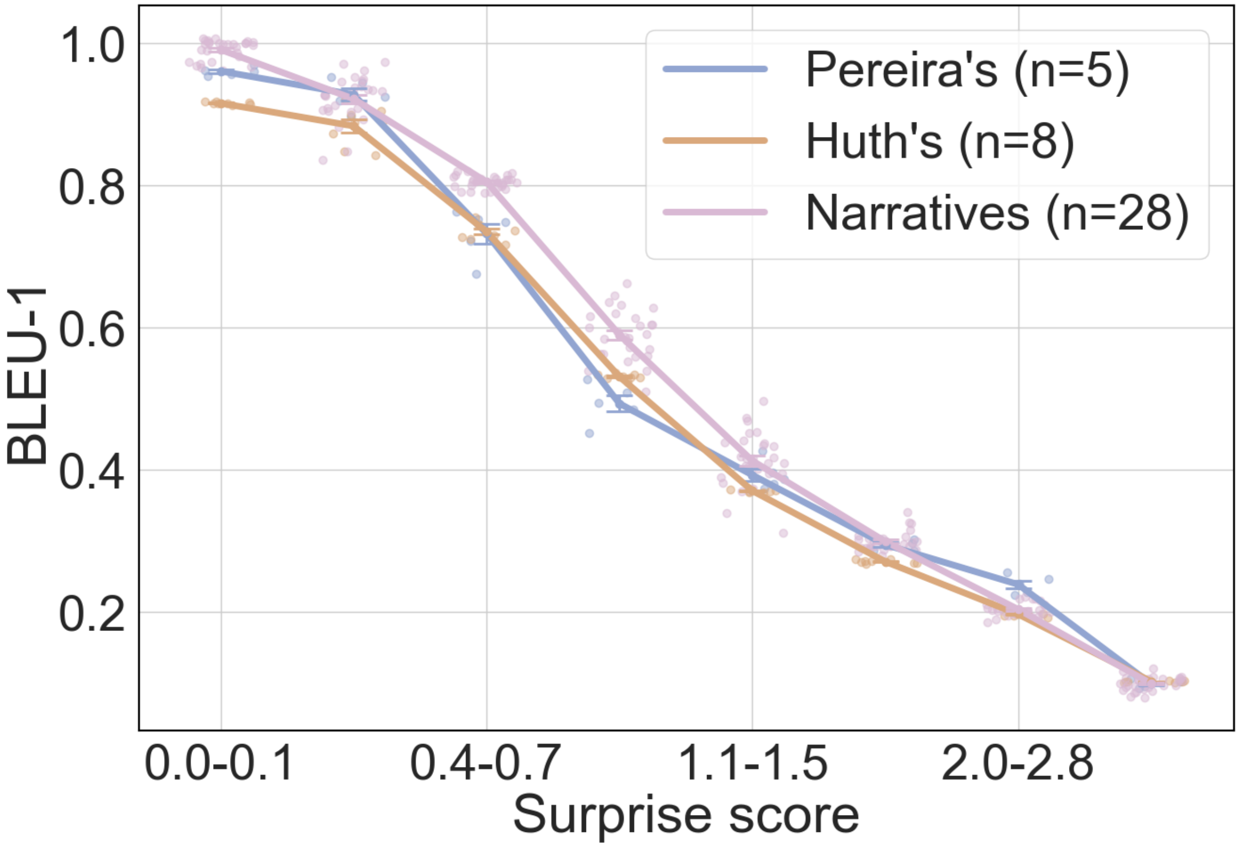


**Fig. 7**: **BLEU-1 score of PerBrainLLM across perceived continuation with different surprise levels.** The Pearson's coefficient $r$ between the surprise levels and the BLEU-1 score in Pereira's dataset, Huth's dataset, and Narratives dataset are -0.67 -0.54, and -0.58, respectively. This observation suggests that with an increased surprise level, it becomes more difficult for the LLM to generate the perceived continuations. Error bars denote mean +/- SEM.

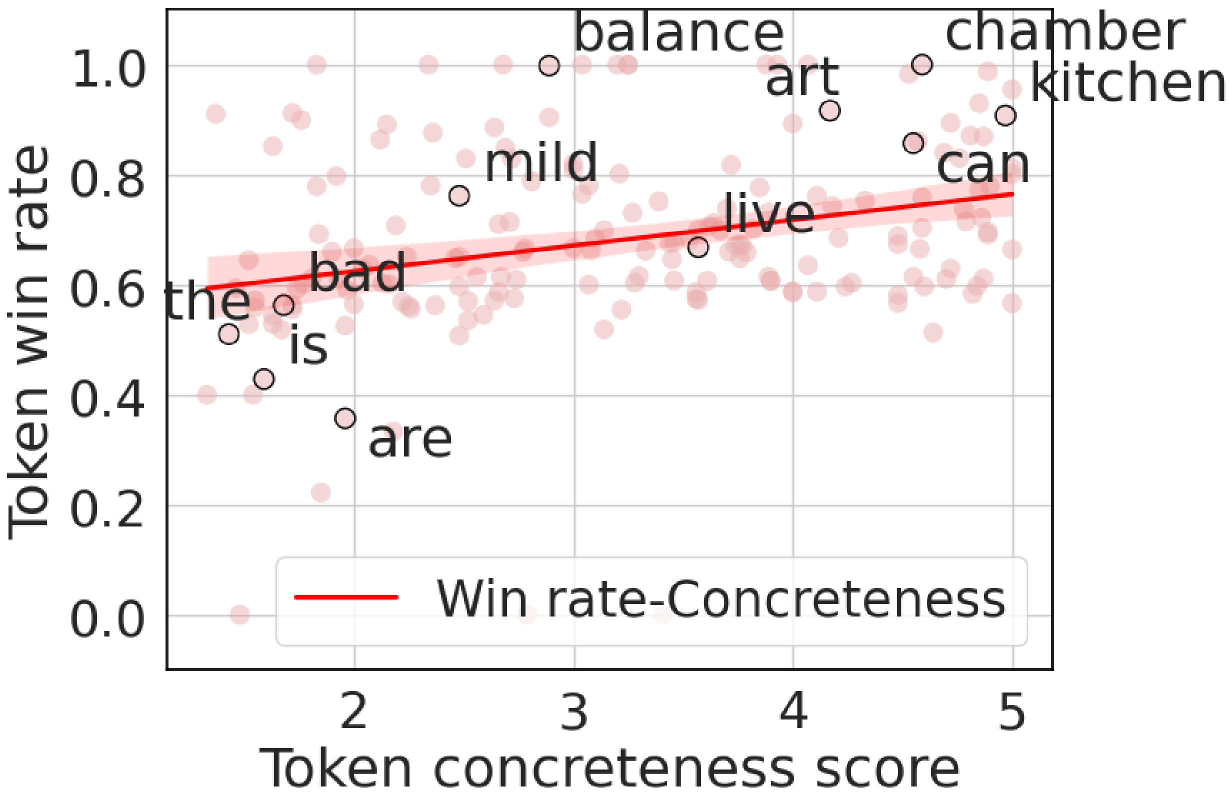


**Fig. 8**: **Scatter plot of win rate versus concreteness scores for 200 randomly selected tokens.** A positive correlation is observed between win rate and concreteness, indicating that tokens with higher concreteness scores tend to have higher win rates.

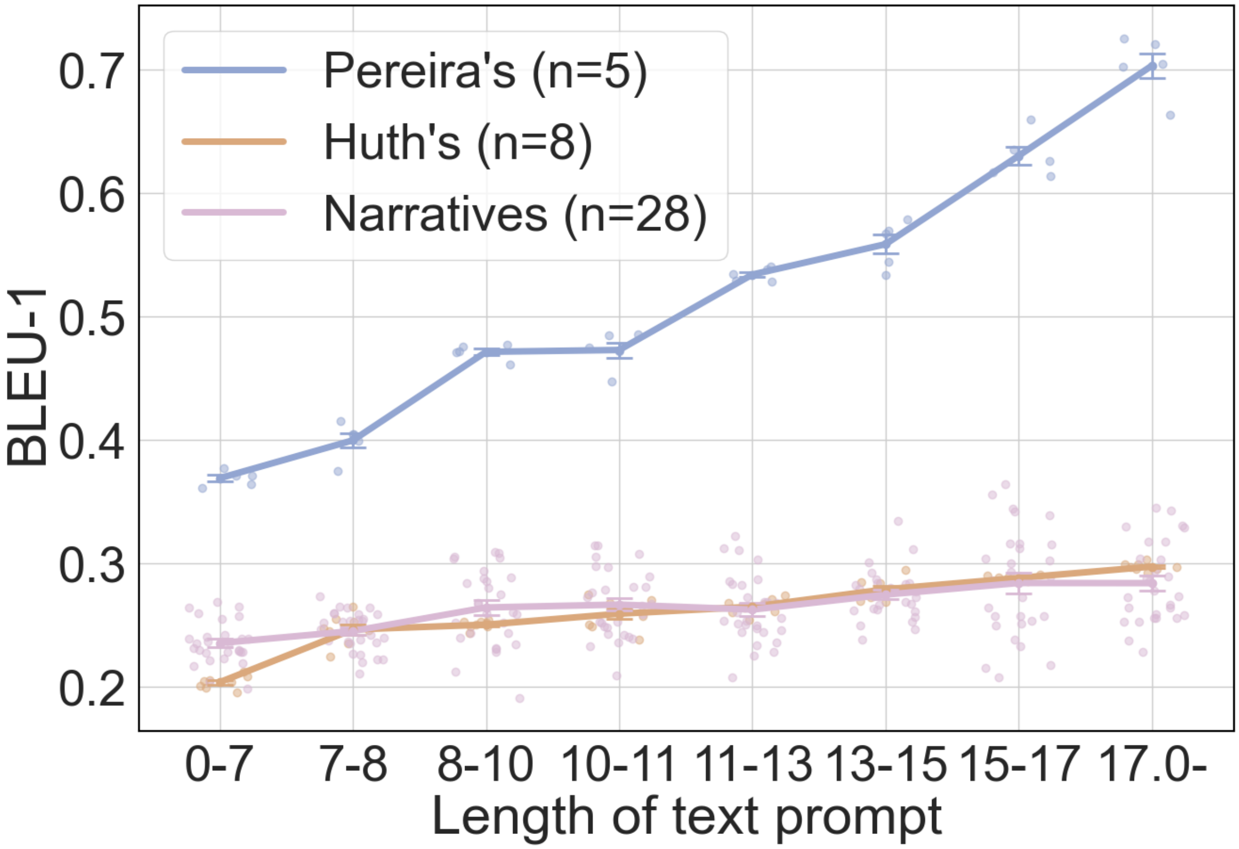


**Fig. 9**: **BLEU-1 score of BrainLLM across text prompt with different lengths.** The Pearson's coefficient $r$ between the length of text prompt and the BLEU-1 score in Pereira's dataset, Huth's dataset and Narratives dataset are significant at 0.27, 0.03, and 0.05, respectively. Pereira's dataset is constructed from Wikipedia and is more similar to the training dataset of a standard LLM than the other two datasets based on speech-style content. Therefore, both the overall performance regarding BLEU-1 and correlation coefficients in Pereira's dataset are higher than the other two datasets. Error bars denote mean +/- SEM.

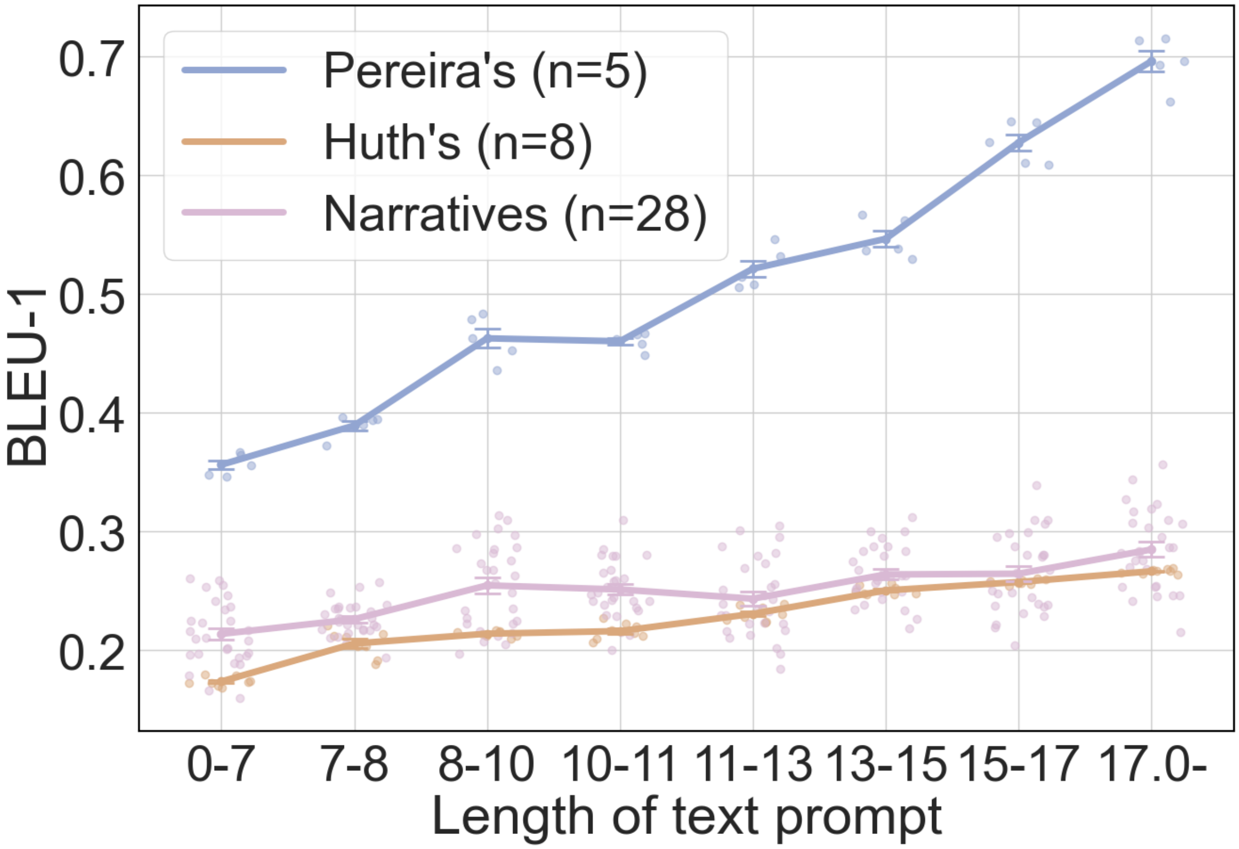


**Fig. 10**: **BLEU-1 score of PerBrainLLM in text prompt with different lengths.** The Pearson's coefficient $r$ between the surprise levels and the BLEU-1 score in Pereira's dataset, Huth's dataset and Narratives dataset are significant at 0.27, 0.02, and 0.03, respectively. Error bars denote mean +/- SEM.

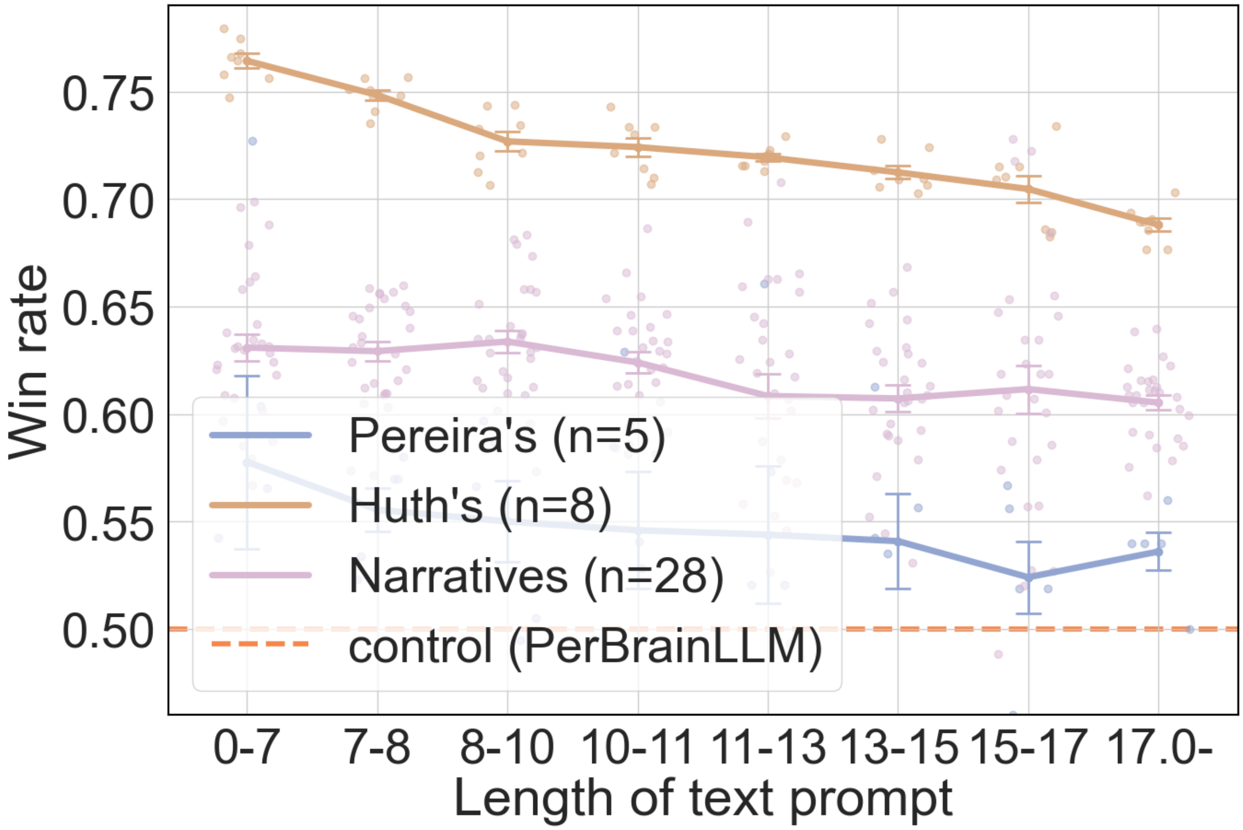


**Fig. 11**: **Win rate between BrainLLM and PerBrainLLM across text prompt with different lengths.** The Pearson's coefficient $r$ between the length of text prompt and the win rate in Huth's dataset and Narratives dataset are significant -0.059 and -0.060, respectively. Both coefficients are statistically significant with p-values of $5e^{-77}$ and $5e^{-40}$, respectively. However, Pearson's coefficient $r$ is not significant in Pereira's dataset (-0.013 with p-values 0.13). This observation could be attributed to the limited sample size of the Pereira dataset, resulting in a scarcity of text prompts of varying lengths. Error bars denote mean +/- SEM.

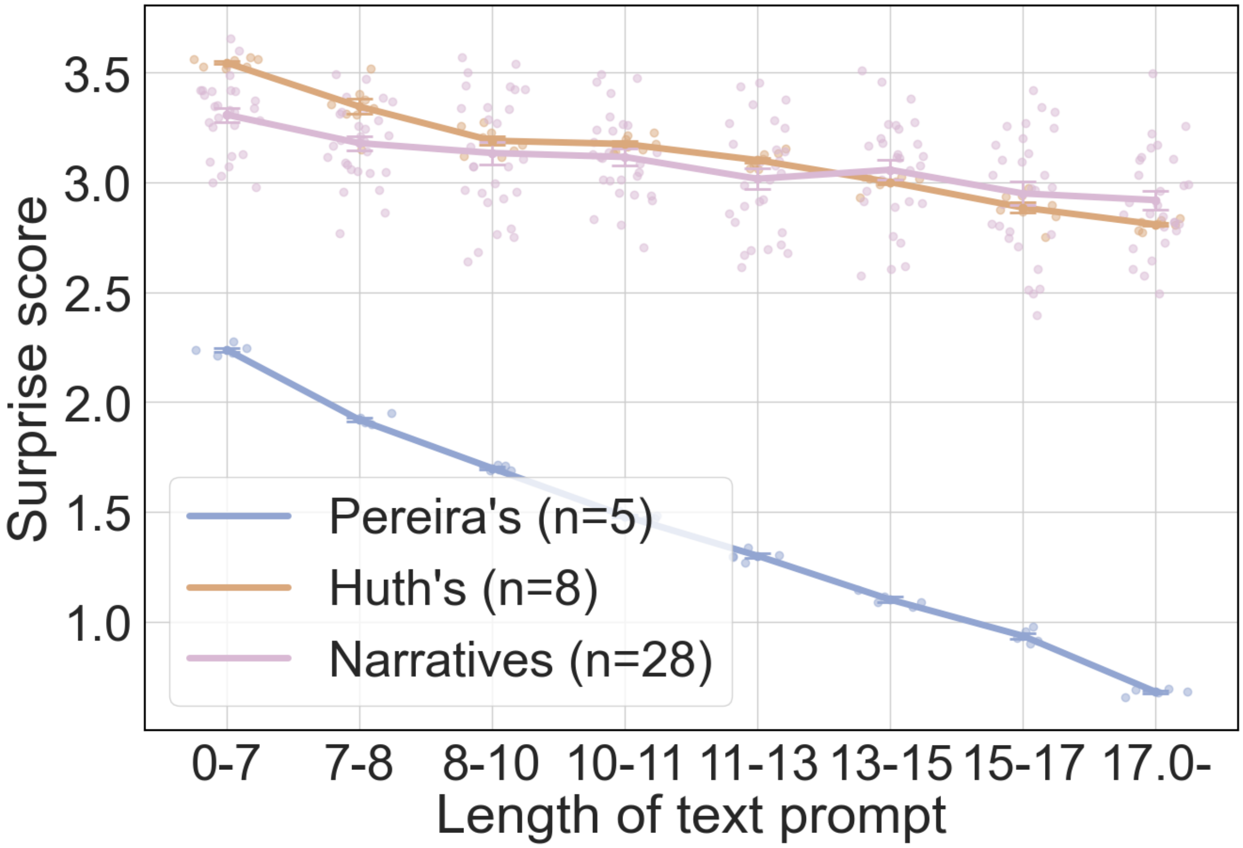


**Fig. 12**: **Surprise score of the perceived continuation across text prompt with different lengths.** The Pearson's coefficient $r$ between the surprise levels and the length of text prompts in Pereira's dataset, Huth's dataset and Narratives dataset are significant with $p < 0.05$ at -0.37, -0.14, and -0.04, respectively. Error bars denote mean +/- SEM.

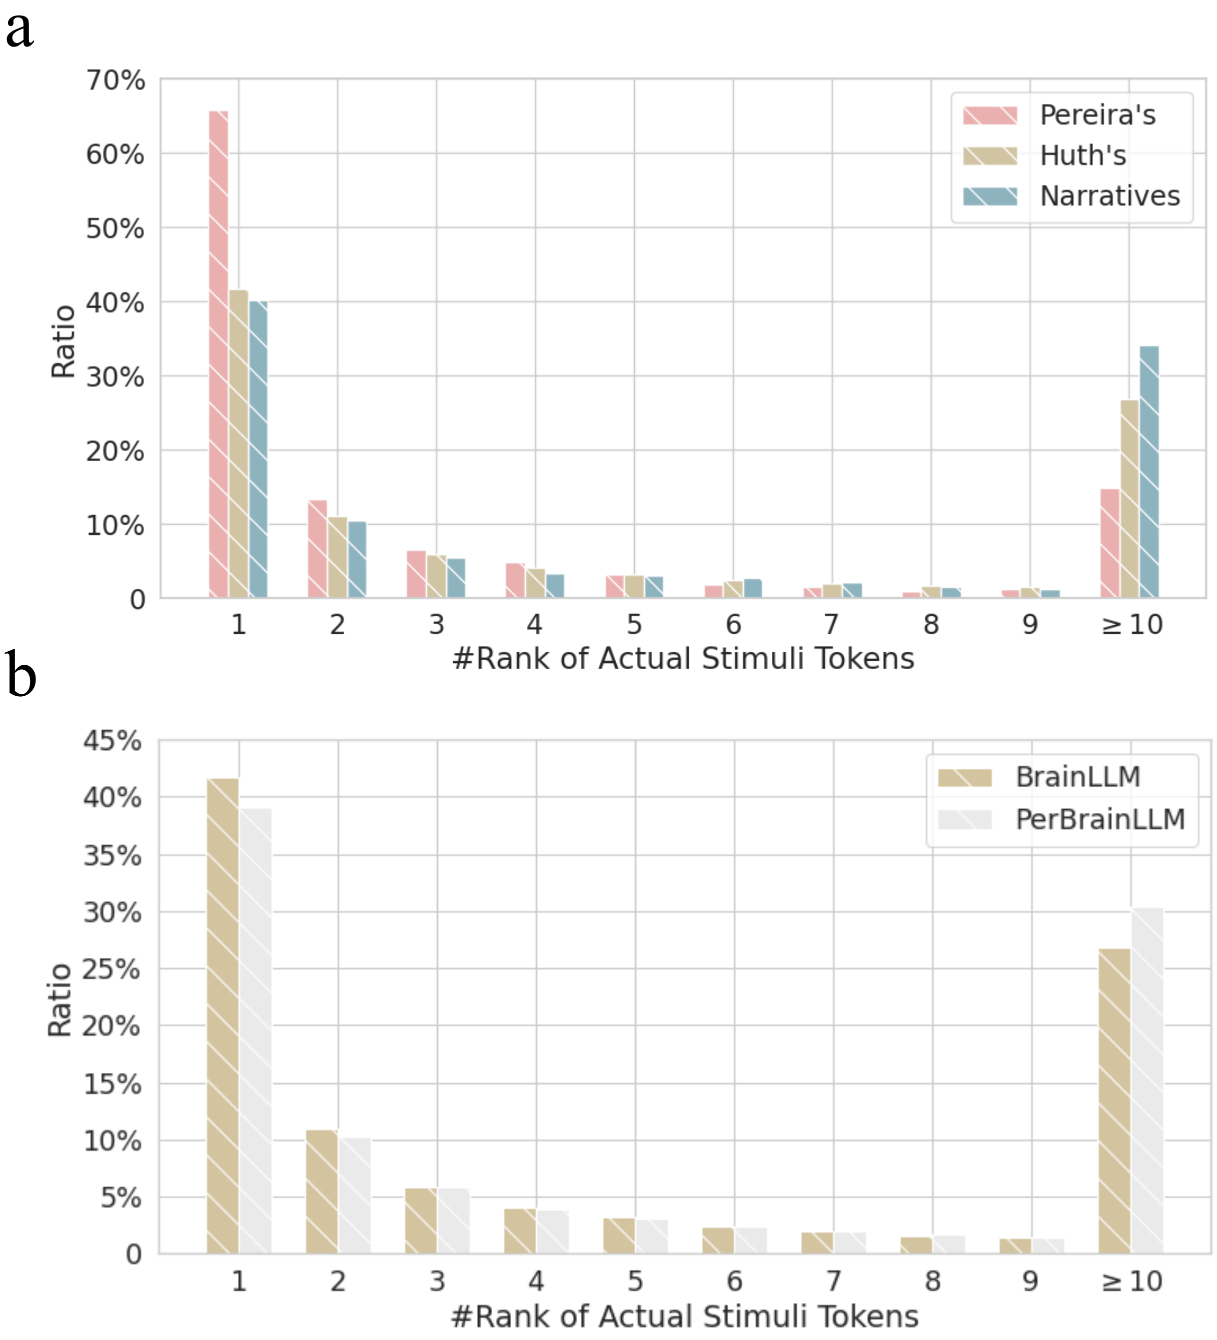


**Fig. 13**: **(a) The rank of token-level perceived continuation in the language generation process with BrainLLM across the three datasets.** A lower rank indicates that the language model considers the token in the perceived continuation as more likely to be generated. Rank 1 indicates that the model accurately predicts the next token. **(b) The rank of token-level perceived continuation in the language generation process with BrainLLM and PerBrainLLM in Huth's dataset.**

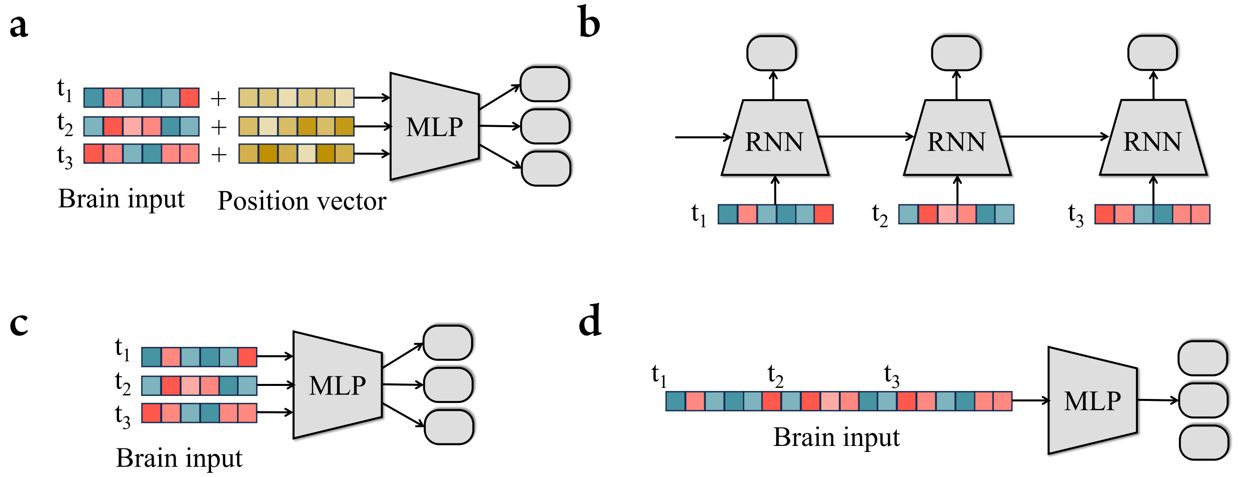


**Fig. 14**: **Structure variants of the brain adapter in BrainLLM. (a)** Multi-layer perception (MLP) with position embedding. **(b)** Recurrent neural network (rnn). **(c)** MLP without position embedding. **(d)** Input concatenation with MLP.

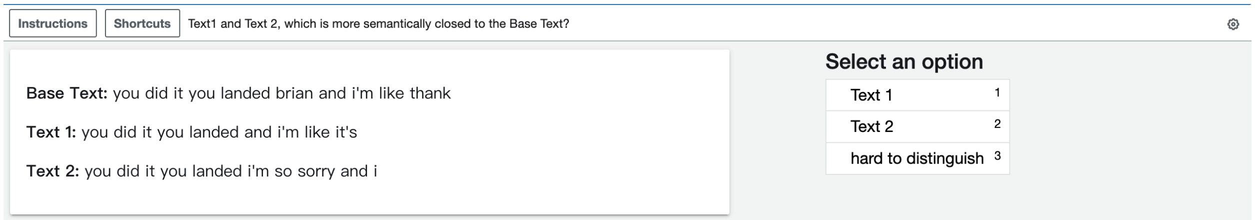


**Fig. 15**: **Screenshot examples of the human evaluation task.** "Text1" and "Text2" are randomly assigned as language generation output from BrainLLM and PerBrainLLM, respectively. "Base Text" is the corresponding perceived continuation. The text prompt is concatenated in front of "Text1", "Text2", and "Base Text" to provide a better context for judging semantic similarity.

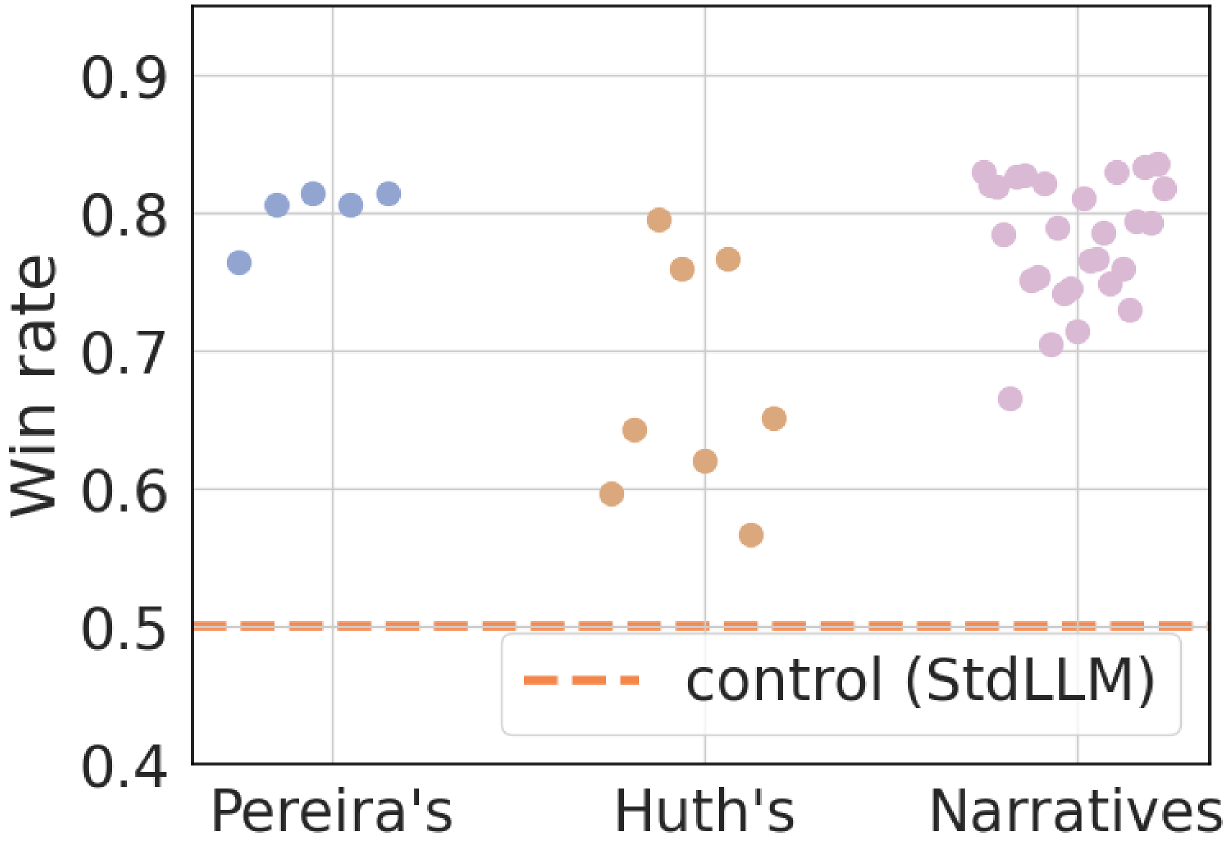


**Fig. 16**: **Win rate of PerBrainLLM vs. StdLLM.** Each dot represents the win rate of a single participant in Pereira's dataset (5 participants), Huth's dataset (8 participants), and Narratives dataset (28 participants).

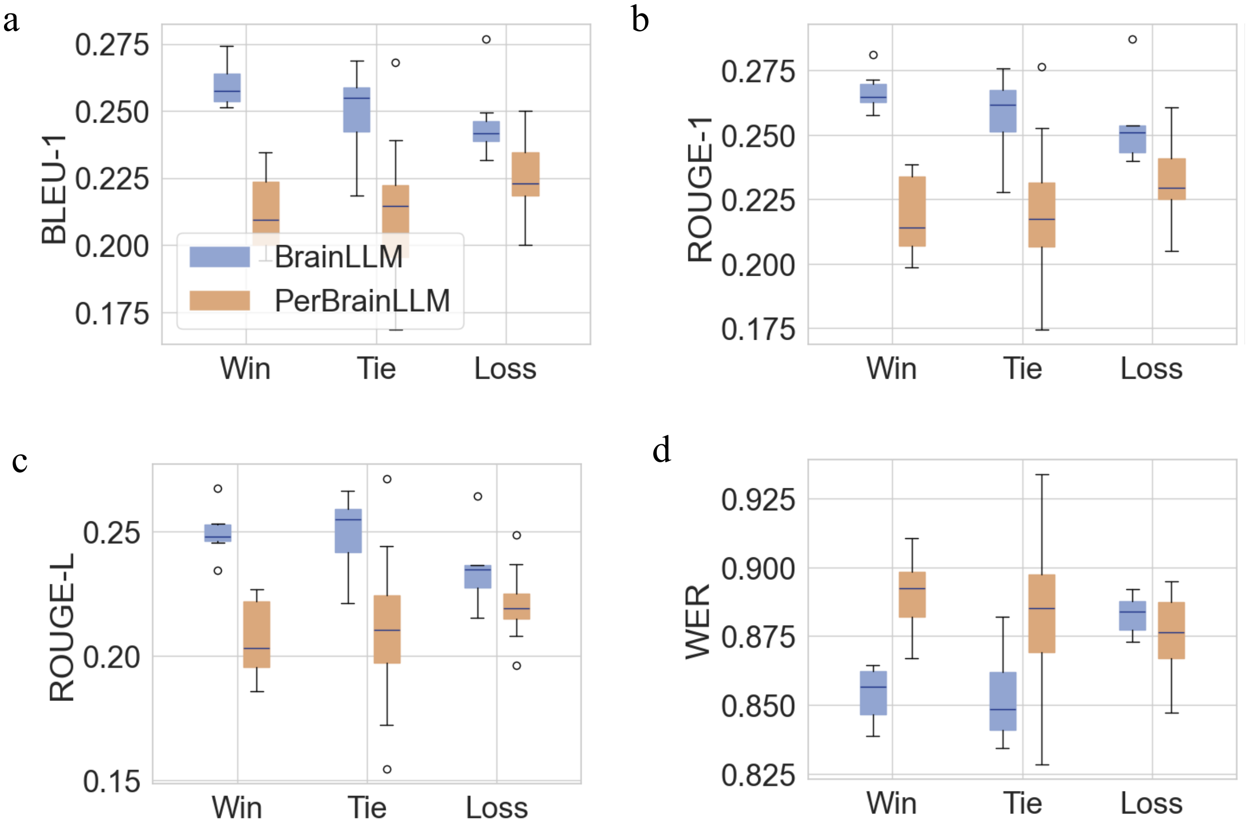


**Fig. 17**: **The language similarity scores in light of the human evaluation results.** The vertical axes of panels **(a)**, **(b)**, **(c)**, and **(d)** represents the language similarity metrics of BLEU-1, ROUGE-1, ROUGE-L, and WER, respectively. The center line, top, and bottom of the box plot represent the group median, 75th percentile, and 25th percentile, respectively. Whiskers are extended to the most extreme data point that is no more than 1.5 $\times$ interquartile range from the edge of the box.

**Table 1: Examples of language generation output from BrainLLM and PerBrainLLM in Pereira's dataset (visual stimuli from Wikipedia content) across various participants.** Blue text indicates the generation output and the perceived continuation are exact match.

| Text prompt | Perceived continuation | Generation with BrainLLM (surprise) | Generation with PerBrainLLM (surprise) | Subject ID |
|---|---|---|---|---|
| *Examples where BrainLLM outperforms PerBrainLLM: Differences in the surprise scores within the top third.* | | | | |
| Electric lawnmowers are better | for the environment because | **for the environment** than gas-powered mowers. (0.7809) | than gasoline-powered ones **because** they are quieter and don't (1.7245) | P01 |
| Drunk driving is the | act of driving under | crime **of driving under** the influence **of** alcohol. (1.5430) | most common cause **of** alcohol-related deaths. (3.3885) | P01 |
| The wind from the | hurricane shook the house, shattering | **hurricane** was so strong that it blew **the** car off (1.7734) | north is cold and dry, while **the** wind from **the** (2.8519) | P01 |
| A wall is a | solid structure that defines | **structure that defines** and sometimes protects an area, such (0.7528) | vertical **structure** made of stone, brick or concrete. (2.2302) | M02 |
| Over the past generation, there has been a | dramatic expansion of legalized gambling. | **dramatic** increase in the number **of** children born to women (1.8443) | huge increase in the number **of** women pilots. (2.6174) | M02 |
| A scientist studies and produces new knowledge | about the physical world. | **about the** natural **world.** (0.6094) | **about the world.** (1.0747) | M02 |
| A wall is a | solid structure that defines | **solid structure that defines** and sometimes protects an area. (0.6725) | **structure that** separates two spaces. (1.6014) | M04 |
| They recorded if they recalled | any **dreams**, and described each | the dream, **and** if so, what it was about. (2.7073) | the information later. (3.3868) | M04 |
| Coffee is a popular | drink in many countries, | **drink in many** parts of the world. Coffee beans (1.0633) | **drink** around the world. Coffee beans are roasted and (1.6215) | M04 |
| Performances are typically given | in an opera house | **in** concert halls or **opera** houses. (1.2981) | **in** theaters or concert halls. (2.0215) | M07 |
| Television content can | be broadcast or received | **be broadcast** live **or** pre-recorded. (1.8579) | **be** entertainment, news **or** education. (2.4874) | M07 |
| That is, a taste bud on the tip of the tongue would respond | only if you were eating something sweet. | to sweet, sour, salty, bitter, or umami. (1.9426) | to a sour taste. (2.2187) | M07 |
| Farms usually have a | house for farmers, a | **house for** the farmer and his or her family. (1.8633) | fence around them to keep livestock in and predators (2.1109) | M15 |
| The polar bear will crawl | quietly forward and freeze in | on its stomach **and** forelimbs to get closer to the (3.3112) | on its stomach to get closer to its prey. (3.5129) | M15 |
| Female mosquitoes bite people | and animals and suck | **and animals** to **suck** their blood. (1.5983) | more often than males. (1.7417) | M15 |

**Table 2: Examples of language generation output from BrainLLM and PerBrainLLM in Pereira's dataset (visual stimuli from Wikipedia content) across various participants.** Blue text indicates the generation output and the perceived continuation are exact match.

*Examples where BrainLLM & PerBrainLLM perform similarly: Differences in the surprise scores within the middle third.*

| **Text prompt** | **Perceived continuation** | **Generation with BrainLLM** (surprise) | **Generation with PerBrainLLM** (surprise) | **Subject ID** |
|---|---|---|---|---|
| Assault rifles can fire in bursts and are | the standard infantry weapon. | used by **infantry** and special forces. (0.9271) | used by **infantry** and special forces. (1.0300) | P01 |
| Tomatoes can be used | to make salads, soup or | **to make** sauces, ketchup and tomato juice. (1.8311) | **to make** sauces, ketchup, salsa and chutney. (1.9277) | P01 |
| Spectacular castles in dramatic locations provide a record of the | stormy history of many regions. | power and wealth **of** medieval rulers. (2.9403) | power and wealth **of** their builders. (3.0320) | P01 |
| Scrubbing a wound with soap or alcohol delays healing, which | increases the risk of infection. | can lead to **infection.** (0.5653) | can lead to **infection.** (0.6313) | M02 |
| A sweater is a heavy garment worn on | the torso for warmth. | **the** upper body. (1.0327) | **the** upper body to keep warm in cold weather. (1.0961) | M02 |
| An elephant has a long nose called a trunk, which | can grab things or food. | it uses for eating and drinking. (3.3345) | it uses for eating, drinking and breathing. (3.3956) | M02 |
| Disposable rubber or latex | gloves are used to shield | **gloves are used to** protect the hands from germs. (1.3808) | **gloves are used to** protect the hands. (1.4422) | M04 |
| We poured the cream mixture into a frozen tub, then start turning the | crank to expose it to the cold. | ice cream maker crank. (2.2776) | ice cream maker on. (2.3339) | M04 |
| Floors may be made | of bare concrete, tile, | **of** wood, stone, tile or carpet. (1.8595) | **of** wood, stone or concrete. (1.9154) | M04 |
| valid -> best features of its predecessors. It incorporates many of the | elements of spoken theatre, such | best features **of** other sports, **such** as soccer and basketball. (2.9760) | best features **of** its predecessors. (3.0300) | M07 |
| A glove is a | piece of clothing that | covering for the hand. (0.7395) | **piece of** leather or cloth **that** covers the hand. (0.7931) | M07 |
| Piranhas are small, | ferocious fish that live | razor-toothed **fish that live** in South America. (1.0150) | carnivorous **fish** with razor-sharp teeth. (1.0666) | M07 |
| A swamp is covered with shallow | water, mud and vegetation. | water **and** dense **vegetation.** (1.1008) | water **and** dense **vegetation.** A swamp can be freshwater (1.1441) | M15 |
| An igloo is a type of shelter made from | blocks of snow by Inuit. | **blocks of snow**. An igloo is usually dome-shaped. (1.6890) | **blocks of snow** and ice. An igloo has a dome-shaped (1.7306) | M15 |
| Walls delineate a building, | support the roof, and | protect it from **the** elements, **and** can be decorated. (1.7052) | protecting it from **the** elements **and** intruders. (1.7460) | M15 |

**Table 3**: **Examples of language generation output from BrainLLM and PerBrainLLM in Pereira's dataset (visual stimuli from Wikipedia content) across various participants. Blue** text indicates the generation output and the perceived continuation are exact match.

| *Examples where BrainLLM underperforms PerBrainLLM: Differences in the surprise scores within the final third.* | | | | |
|---|---|---|---|---|
| **Text prompt** | **Perceived continuation** | **Generation with BrainLLM** (surprise) | **Generation with PerBrainLLM** (surprise) | **Subject ID** |
| Cats can hunt mice | or birds, but are | , rats, **birds** and other small animals. (1.8762) | , rats and other small animals. (1.7944) | P01 |
| The piano repertoire is large and famous pianists | can give solo concerts. | have written many original compositions. (2.3033) | often perform in **concerts.** (2.2118) | P01 |
| Retaining walls provide a | barrier to movement of | **barrier** against erosion and flooding. (1.9046) | **barrier** against erosion and flooding. (1.8184) | P01 |
| A sweater that opens down the front | is called a cardigan. | **is called a cardigan.** (0.3550) | **is called a cardigan.** (0.2818) | M02 |
| Raspberries are eaten | by themselves or cooked | fresh **or** used to make jams and desserts. (2.4154) | fresh **or** made into jams, pies and other desserts. (2.3410) | M02 |
| A horse is a | large hoofed mammal with | **large mammal with** four legs and a long tail. (0.7095) | large, **hoofed mammal with** a long neck and mane. (0.6265) | M02 |
| Blenders have a glass | or plastic container with a | **or plastic container with a** rotating blade. (0.7227) | **or plastic container with a** rotating blade. (0.6573) | M04 |
| A glove is a | piece of clothing that | covering for the hand, usually made **of** leather. (0.8059) | covering for the hand. It can be made **of** (0.7375) | M04 |
| Some patients go there | for specialist diagnosis or | voluntarily, while others are involuntarily committed. (2.3428) | **for** treatment of chronic diseases. (2.2665) | M04 |
| A sweater is a heavy garment worn on | the torso for warmth. | **the** upper body. (0.9449) | **the** upper body to keep warm. (0.8729) | M07 |
| During times of attack, peasants, | livestock, and property could be brought | merchants **and** priests would flee. (2.6384) | merchants **and** craftsmen **could be** conscripted. (2.5643) | M07 |
| The type of forest | depends on temperature and | is determined by climate, soil **and** topography. (2.1033) | **depends on** the climate **and** the type of trees (2.0256) | M07 |
| Cruise ships are floating hotels that | take people between cities. | travel the world's oceans and seas. (3.6322) | travel the world's oceans and seas. (3.5694) | M15 |
| Lettuce is considered fairly | easy to grow and | low in nutritional value, but it is a good (0.7081) | low in calories **and** is a good source of (0.6411) | M15 |
| The market for admission to law school and for | new lawyers could eventually crash. | **lawyers** is very competitive. (3.1436) | jobs as **lawyers** is very competitive. (3.0660) | M15 |

**Table 4**: **Randomly sampled examples of language generation with BrainLLM and PerBrainLLM in Huth's dataset.** Blue text indicates the generation output and the perceived continuation are exact match. These samples were selected from participants 1, 2, and 3.

| Text prompt | Perceived continuation | Generation with BrainLLM (surprise) | Generation with PerBrainLLM (surprise) | Subject ID |
|---|---|---|---|---|
| *Examples where BrainLLM outperforms PerBrainLLM: Differences in the surprise scores within the top third.* | | | | |
| you see in the morning I'll be paroling from | state prison after twenty | the **state** penitentiary where I've been incarcerated for a (2.4710) | the beach and I'll see you then thank you (4.5921) | 1 |
| around and we sort of spent the morning like this and it was all really um just | fine and then um | very peaceful **and then** in the afternoon we went (2.2719) | being in awe of what we were seeing **and** (5.3981) | 1 |
| nee use to know the mortality rates hence tell you how | much premium you need to pay | long you're going **to** live and hence how **much** money **you need to pay** (1.3060) | long you're gonna live uh and i was like eighty per (3.5567) | 1 |
| was trying to make my mom look bad in front of the teachers to like deflect | um y you know | the blame **um** and uh **you know** it was (3.1762) | some of the blame from her onto me and (5.9958) | 1 |
| let it come wait for it wait for it i | see the horizon coming up my feet get a little | 'm at **the** top of **the** arc i'm over **the** ocean i'm looking down and (2.9004) | was like no i'm not gonna wait for it and he said well then you (5.1265) | 1 |
| would come pick us up and we had to do that twice and if you did that twice | successfully you pass the water | **you** were out of **the** navy and i didn't want (3.9887) | in a row **you** were uh suspended from school uh (6.7814) | 2 |
| where i pick up my bag | and i replace the handset | **and** my phone **and i** walk out of **the** shop (2.4662) | **and** i'm gonna go back to new york um **and** (4.9229) | 2 |
| that everything happened in slow motion | the voice in my head asks me | and then all of a sudden i look up and i see (2.5491) | nd um and so i was **in the** hospital for a couple (4.9326) | 2 |
| was because it was also where we kept | all of the family photos | **all of** our **family** pictures and i had a lot (1.6215) | **the** goats and **the** pigs and **the** chickens and **the** (3.8364) | 2 |
| with forty three other new astronauts but we weren't really | astronauts yet we were | **astronauts yet we were** trainee **astronauts** and **we** had (0.2619) | talking about that **we were** talking about the fact (2.4186) | 2 |
| been tough immediately we start to reminisce about our thirty second relationship i didn't think that was gonna happen | me neither oh man that was close | i didn't think **that was** gonna happen but it did and we (4.5486) | but it did and then we start to reminisce about the fact (5.7116) | 3 |
| what insurance companies | nee use to know | don't want you **to know** is that if you (5.6416) | don't do is they don't tell you what **to** (6.5533) | 3 |
| but no you had to be topless for an entire | song and i'm like oh no but i | day **and i'm like** well that's not gonna work for me so **i** (1.7108) | day **and** then you had to be nude for an entire day **and** (2.5826) | 3 |
| requests so we said that | we preferred a boy | we'd be happy to do that and then **we** (3.9074) | 's great we'd love to do that and he (4.7590) | 3 |
| of the organization it doesn't mean that every storm trooper gets personal one on one time | so i try to | with luke skywalker and **so** i'm like you know (2.9701) | with darth vader but it does mean that every (3.7780) | 3 |

**Table 5: Randomly sampled examples of language generation with BrainLLM and PerBrainLLM in Huth's dataset.** **Blue** text indicates the generation output and the perceived continuation are exact match. These samples were selected from participants 1, 2, and 3.

| *Examples where BrainLLM & PerBrainLLM perform similarly: Differences in the surprise scores within the middle third.* | | | | |
|---|---|---|---|---|
| **Text prompt** | **Perceived continuation** | **Generation with BrainLLM** (surprise) | **Generation with PerBrainLLM** (surprise) | **Subject ID** |
| saleswoman and it started to get confusing like which hat i was wearing at which time until | one day i was in | **one day** i'm **in** the dressing room and there's a (1.2526) | finally **i** realized that **i** **was** the patient and she (1.7785) | 1 |
| and it's late spring and i go visit some | friends at princeton and yet again i get | **friends** in new york city **and** i'm staying with a friend of a (2.6285) | of my cousins **and** they're all like oh my god it's so great (3.1530) | 1 |
| mine sends me lolita which i had never read before which is not the best sort of | reading material when there's like twelve and | lolita to read because it's the one that's all about nymphets **and** (3.2295) | book to read **when** you're going through something **like** this but i (3.7540) | 1 |
| into a raft signal for help and they | would come pick us up and we had to do that twice | 're going **to come and** rescue me **and** i'm going **to** be fine **and** i'm going **to** (2.0334) | 're not going **to** be able **to** hear you over the sound of your own screaming but (2.5564) | 1 |
| in full gear flight | suit boots and helmet | **suit helmet** oxygen mask goggles gloves **boots** parachute **and** (1.2413) | suits helmets goggles oxygen masks **and** all the rest (1.3972) | 1 |
| because i i would i would like to say because of the uh incredible amount of love | that you have for them but that's not | **that** my parents had **for** me **but** i think it was more because (1.4390) | and affection **that** i had **for** her **but** it was probably more because (1.8998) | 2 |
| assistants to madame diof who had all gathered around and we sort of spent the morning like this | and it was all really um just | **and** then we went back to the hotel **and** had lunch **and** (3.2112) | **and** then we had lunch **and** then we sort of spent the (3.6719) | 2 |
| the artist never quite pinned down never | quite in a relationship and and you have | **quite** figured out what was wrong with me but i knew that there (3.4595) | **quite** figured out what was wrong with me **and** i think that's probably (3.9192) | 2 |
| headphones still there are the headphones still there i i'm on the verge of a nervous | breakdown when finally one of the president's aides | **breakdown** and then i hear a knock on **the** door it's **the** president (1.8259) | **breakdown** i'm on **the** verge **of** a nervous **breakdown** i'm on **the** verge (2.2814) | 2 |
| they inject something into your ankle like an iodine solution and then you they lay you | on a table and you get slid into | down **on a table and** they cut **you** open from your pubic area (2.0988) | down **on a table and** you're strapped to the **table and** then they (2.2224) | 2 |
| and and bird watching camps there's | even a camp where you can dress up in armor | all kinds of camps out there and i went to **a** lot of them and (2.1303) | also **a** nature center that's open to the public and it's run by volunteers so (2.2510) | 3 |
| and the smith corona my smith corona even and to put them all in the front yard next to the rock | garden not too close to the maple tree | ing chair and i'm sitting in **the** rocking chair with my smith corona (3.0263) | ing chair on **the** front porch and i'm sitting in **the** rocking chair (3.1943) | 3 |
| what to do when a woman taps you on the | shoulder at a crowded restaurant and demands | **shoulder and** tells you that she's the first lady of the united (2.0442) | **shoulder and** she's like oh my god i'm so sorry i didn't (2.2111) | 3 |
| their income their status all of our fortunes were tied in together | and i thought but is this | **and** so it was a very intimate experience **and i** think (3.1160) | **and** so i'm sitting there **and** i'm like oh my god (3.2820) | 3 |
| problem i reach down tie that garbage bag up throw it over my | shoulder and out to the front door i | **shoulder and** i'm walking **out** of **the** house when all of a sudden (2.1623) | **shoulder and i** walk **out** of **the** house **and i** get in my (2.1793) | 3 |

**Table 6**: **Randomly sampled examples of language generation with BrainLLM and PerBrainLLM in Huth's dataset.** Blue text indicates the generation output and the perceived continuation are exact match. These samples were selected from participants 1, 2, and 3.

| *Examples where BrainLLM underperforms PerBrainLLM: Differences in the surprise scores within the final third.* | | | | |
|---|---|---|---|---|
| **Text prompt** | **Perceived continuation** | **Generation with BrainLLM** (surprise) | **Generation with PerBrainLLM** (surprise) | **Subject ID** |
| fist bump in the hallway or someone else got invited up to play cards on air force one a and the moral was | always the same any moment could be the | don't get your hopes up **the** white house is a big place and (2.5582) | **always the same** you never know when it's going to **be** your last (2.0025) | 1 |
| it's like embarrassing you know i mean | cg i don't know like | **i don't know** if you've ever been in this situation (4.5028) | it's embarrassing that i'm crying but **i** couldn't help it (3.9436) | 1 |
| but a lot | of them are adults | **of** people who work in washington don't know what (3.8812) | **of** people have asked me over the years why (3.2763) | 1 |
| but i can see myself in my kid and | i i can see myself sitting at the | **i can see** my dad in my kid and it's just a beautiful (2.7459) | **i can see myself** in my wife and **i can see myself** in (2.0235) | 1 |
| stick figures every forty five seconds because that's how fast the poses are | every forty five seconds and | changing **and** i'm thinking if i can do this then (2.1718) | so i'm doing stick figures **every forty five seconds** for (1.4118) | 1 |
| i did a sold out | reading at foyles in london | show **in** new york and then i went to **london** (2.7226) | show **at** carnegie hall **in** new york city and i (2.1535) | 2 |
| weber's farmhouse i met a very pretty girl | she was his assistant and she gave me her phone | who **was** a photographer's **assistant and** uh we fell in love **and she** had an (3.2647) | who **was** the daughter of the man who owned the farm **and she** told **me** (2.6886) | 2 |
| center he was away on work experience and he'd given me the keys to his flat which was great for me | because i lived off main campus | **because** i'd been living in a hostel for the last couple (4.3534) | **because** i'd never been in a flat before uh and he'd (3.7667) | 2 |
| and clothes from the salvation army i had moral obliga | um objections to wearing make up | tions but i didn't have a lot of money **to** spend (3.6350) | i had a moral obligation **to** tell her that she was (3.0323) | 2 |
| like you know well i don't think it's worth | doing but you know i | the risk so we're gonna have to go with plan (2.5767) | it **you know i** don't think it's worth it and (2.2407) | 3 |
| fully immersed and then my uncle al who never | ever played with us ever | swam a day in his life comes up to me (3.9922) | smoked a cigarette in his life he's like you know (3.6355) | 3 |
| out to yell at us but they start fake smiling and trying to act all normal | and my aunt momo | **and** i'm like oh **my** god they're trying to (4.3839) | **and** i'm like oh **my** god they're not gonna (4.0172) | 3 |
| going to ruin it i wanted to be him | and then when they leave | i wanted to be like him i wanted to be (3.8429) | i wanted to be that guy **and** so i'm like (3.4656) | 3 |
| mediums with which they excel | and i'm just standing there like | **and** so **i'm** sitting in my office one day **and** i (2.1645) | **and i'm like** oh my god this is the best thing (1.7781) | 3 |

**Table 7**: **Randomly sampled examples of language generation with BrainLLM and PerBrainLLM in Narratives dataset.** These samples were selected from participants who have participated in at least 4 fMRI scans, including 016, 052, 065, 066, 075, 084, 106, and 111. **Blue** text indicates the generation output and the perceived continuation are exact match.

*Examples where BrainLLM outperforms PerBrainLLM: Differences in the surprise scores within the top third.*

| **Text prompt** | **Perceived continuation** | **Generation with BrainLLM** (surprise) | **Generation with PerBrainLLM** (surprise) | **Subject ID** |
|---|---|---|---|---|
| how illegal that probably was | and she says | **and she says** (1.396) | for him to (4.923) | 016 |
| um um she was like petite i could have | folded her up and put her my pocket she looked | picked **her up** with one hand **and put her** in the trunk of **my** car (2.3750) | **put her** in the trunk of **my** car **and** driven **her** to work every day (2.6931) | 016 |
| stop that's what kills you and so i | lock eyes with her and i | 'm standing there **and** i'm looking at this guy **and** i'm (2.4197) | did **and** then **i** went back to my apartment which was (2.6821) | 052 |
| yeah she quickly learned to hold her own bottle at | two months her eyes would | the age of six **months** and she's been drinking cow's (3.4729) | arm's length and drink from it without spilling a drop (3.9846) | 052 |
| hand and will not let it go | I'm so glad you're | **I'm so glad you're** (2.835) | **I'm** sorry I'm so (4.054) | 065 |
| stop that's what kills you and so i | lock eyes with her and i | 'm standing there **and** i'm looking at **her and** she's looking (2.5705) | 'm not going to stop i'm going to keep right on (3.6535) | 065 |
| I think several days of the | study and then she | experiment **and then** we (3.181) | same thing I think (5.854) | 066 |
| romanian gymnast | and she says you know okay y you | **and** she's in her early twenties **and** she's very attractive **and** she's wearing (3.6662) | ics what do **you** mean romanian gymnastics we've been doing romanian gymnastics for (5.5957) | 066 |
| um fruit carts and stuff | and then um he | like that **and then um** he's just kind of (1.5774) | margaret says i don't know what you're talking about (5.2690) | 075 |
| wait no not yet this time he is sent to give | uh her like the | **her** a message um and so sherlock tells him (2.7693) | a speech at columbia he's on **the** front page (6.0884) | 075 |
| somewhere so she's home what a rat | race honest to god | what a rat i'm going **to** kill that **god** (3.1600) | in new york you know she's like a rat (4.4346) | 084 |
| very tough situation the guy's obviously going through absolute the phone | suddenly rang the gray | **rang** agony and he's got to get out of (4.2608) | 's ringing agony and he picks up **the** phone (5.2294) | 084 |
| tell the truth | is it going to do you any good | i don't know what you're **going to do** about **it** but i'm not (1.9322) | **you** know i've been in new york for thirty five years and i've (2.9949) | 106 |
| tight her open eye very however large | and so blue as to appear | **and** very **blue** she said you know what i'm going **to** (2.7501) | **and** i'm not sure if it's a good thing or a (3.7188) | 106 |
| situation the guy's obviously going through absolute the phone | suddenly rang the gray | **the gray** haired man said i don't know what (2.5783) | and he's like i'm going insanity you know **the** (7.6719) | 111 |
| wake you the gray haired man glanced | briefly left at the girl | over his shoulder **at the** gray haired woman who had (3.6355) | up **at** me and he said you know i've been (5.2840) | 111 |

**Table 8**: **Randomly sampled examples of language generation with BrainLLM and PerBrainLLM in Narratives dataset.** These samples were selected from participants who have participated in at least 4 fMRI scans, including 016, 052, 065, 066, 075, 084, 106, and 111. **Blue** text indicates the generation output and the perceived continuation are exact match.

*Examples where BrainLLM & PerBrainLLM perform similarly: Differences in the surprise scores within the middle third.*

| **Text prompt** | **Perceived continuation** | **Generation with BrainLLM** (surprise) | **Generation with PerBrainLLM** (surprise) | **Subject ID** |
|---|---|---|---|---|
| and bob still | lived in our building i would | to this day doesn't know what **i** was talking about but (3.2736) | to this day is the only person i've ever met who (3.3426) | 016 |
| work for the new york times and i was working a story one time about money | laundering on a little | **laundering** in the cayman islands and i was talking (1.9536) | **laundering** in the cayman islands and so i went (2.0190) | 016 |
| over looked at it like antarctica but of course | that's my space was always | i didn't know any of this at the time and (3.5026) | i'd never been to antarctica so i didn't know what (3.5060) | 052 |
| that the movement didn't quite look perfunctory | she cleared her hair back | i mean it looked as if **she** were really trying (4.5558) | i mean it didn't look as if **she** was just (4.6744) | 052 |
| they probably all hopped in a cab and went | down to the village for a couple of | home **to** their wives and kids and **the** next morning they got up (1.8726) | home **the** next morning when i got **to** work there was **a** note (2.0255) | 065 |
| maybe there really was some sort of explosion that started this dreaming | well there will be an explosion down at | business but i don't think so i think it's all part of some(3.1162) | but i don't think so i think it's the same thing that's been (3.2655) | 065 |
| me and toward the end of this run i was out at a | bar one night and i saw | **bar** with a bunch of my friends **and** we're all drinking (1.4914) | **bar** **and** **i** was drinking with a bunch of my friends (1.6697) | 066 |
| jim we were just talking | about how you always | **about** the fact that you're going to be a (2.2731) | **about** this the other day and i said to (2.4484) | 066 |
| walked out of a marriage or something or | is an alcoholic or both | walked out of a relationship **or** something like that and (2.7615) | someone i don't know margaret says she doesn't want to (3.1711) | 075 |
| tense interaction | there he asks uh | between the two of them and then **uh** there's (2.8394) | between the two of them and then um sherlock (3.2370) | 075 |
| and then | she says don't worry i'll | he **says** you know what i'm going to do is (1.8448) | he said you know what i'm going to do i'm (1.9885) | 084 |
| get this guy so we took the very brief eight and a start chatting and it's like half minute ride from | unbelievable and uh standing still on the ground to | new york **to** boston **and** i'm sitting there **and** i'm talking **to** this guy (3.1790) | bob's apartment **to** my apartment **and** we're chatting away **and** he says you know (3.3136) | 084 |
| i say this in all sincerity will you get undressed and get into | bed like a good guy | **bed** and i'll be there in **a** few minutes he (2.8405) | the shower and i'll be there in **a** couple of (2.9818) | 106 |
| very nearly do every | night when i get home | single one of them and **i** think that's what makes (2.5423) | single one of those things and i'm not going to (2.6685) | 106 |
| to teach you how to do a drop and roll which is this maneuver you do when you land it's where you | basically it's what it sounds like you drop and | land on your side **and** **you** roll out of the way so that **you** (1.8660) | land on your side **and** then **you** roll away from the impact so that (2.1725) | 111 |
| hop on the bus gus and i | think nice we have something in | 'm like oh my god he's going to kill me i'm (5.0009) | 'm like you know what i'm going to do i'm going (5.3027) | 111 |

**Table 9**: **Randomly sampled examples of language generation with BrainLLM and PerBrainLLM in Narratives dataset.** These samples were selected from participants who have participated in at least 4 fMRI scans, including 016, 052, 065, 066, 075, 084, 106, and 111. **Blue** text indicates the generation output and the perceived continuation are exact match.

*Examples where BrainLLM underperforms PerBrainLLM: Differences in the surprise scores within the final third.*

| **Text prompt** | **Perceived continuation** | **Generation with BrainLLM** (surprise) | **Generation with PerBrainLLM** (surprise) | **Subject ID** |
|---|---|---|---|---|
| killed they had this guy shot you know one of those stories | the guy's found dead under a | that's and i was like you know it's kind of hard (2.8172) | that's just too good to be true and so i called (2.6888) | 016 |
| without a for most of it as far as i'm | concerned and i i | **concerned** you know i'm not going to be able (2.3960) | **concerned** you know i'm not going to be able (2.2632) | 016 |
| and said god i don't know | i mean what do you think | **i** don't know **what** to make of it mr henry you're (2.0291) | what's the matter with me **i** don't know what's the matter (1.9017) | 052 |
| intellectual that's the funny part that's the hilarious part | she reads the theatrical | that's **the** god damn funniest part of all i (4.6749) | that's **the** funniest thing i've ever heard in my (4.5382) | 052 |
| tell the truth is it going to do you any good | to sit around and stew | i don't know what you're trying **to** do but it (3.0622) | **to** tell the truth you're not going **to** believe me (2.9767) | 065 |
| won't you let me | buy some of them for you huh | tell **you** what's going to happen first **of** all they're going to (3.4254) | get a word in edgewise will **you** just let me tell **you** (3.3369) | 065 |
| know i'm not sure i was looking for a fuse and i thought maybe i'd dropped one | under the boathouse so i scratched | on **the** floor but **i** didn't find one and then all (3.7047) | on **the** floor or something and **i** was looking for it (3.5558) | 066 |
| place the gray haired | man said and slowly moved his | **man** looked up from **his** typewriter **and said** good morning i'm (2.9905) | man's voice came out of the darkness he was standing in (2.7964) | 066 |
| on the way there | they have a conversation in the cab | and then uh he's talking to her about **the** case that they're (3.1337) | um sherlock and watson are talking about this case that they've been (2.9230) | 075 |
| flier elated graduating and gown and all they tape his | face next to the weathered | diploma **to the** refrigerator i'm so proud of you margaret (3.9406) | flier **to the** bulletin board in **the** lobby of her (3.7263) | 075 |
| ceiling uh didn't she leave with you no christ you didn't see | her leave at all then w | **her** you didn't see **her at all** did you no i (3.8462) | **her** did you she didn't come back with you i don't (3.7091) | 084 |
| trouble and only things like | um and bob realized alpine mountains or | that **and** so i said you know what i'm going to do (4.8688) | that you know **and** so i'm sitting there **and** i'm looking at (4.7052) | 084 |
| and get away with it because it's written into the | constitution that you can't prosecute | **constitution** of the united states **that you can't** kill somebody (1.3103) | **constitution** of the united states **that you can't** be tried (1.1602) | 106 |
| i'm the one who put him away crawled up | inside squeezed inside this | to the top of the building and looked down (4.1327) | on the ceiling and crawled out of the apartment (3.9751) | 106 |
| tub doing standing | with all this water and why are | up in the tub doing standing up in the tub doing standing (4.2724) | up in the bathtub **and** i was like oh my god **this** (4.0076) | 111 |
| and i guess i | didn't know the protocol of | don't **know** if this is true or not but one (2.9560) | don't **know** if this is true or not but i (2.6666) | 111 |

**Table 10**: **A summary of brain decoding research using LLMs with different validation setups.** TF, FTC, and TC indicate teacher forcing, full text construction, and text continuation, respectively.

| Model | Validation | Dataset | Performance (%) |
|---|---|---|---|
| Wang et al. [21] | TF | ZuCo | BLEU-1=40.1, ROUGE-1=30.1 |
| UniCoRN [22] | TF | ZuCo | BLEU-1=35.9, ROUGE-1=39.1 |
| | TF | Narratives | BLEU-1=62.9, ROUGE-1=59.5 |
| DeWave [10] | TF | ZuCo | BLEU-1=41.4, ROUGE-1=30.7 |
| NeuSpeech [23] | TF | Schoffelen | BLEU-1=78.1, ROUGE-1=83.7 |
| | FTC | Schoffelen | BLEU-1=67.8, ROUGE-1=81.2 |
| MAPGuide [24] | FTC | Huth's | $\text{BLEU}_{\text{zs}}$=10.91, $\text{METEOR}_{\text{zs}}$=11.92 |
| Tang et al. [14] | FTC | Huth's | BLEU-1=24.09, WER=92.02, METEOR=16.67 |
| PREDFT [25] | FTC | Huth's | BLEU-1=25.98, ROUGE-1=19.61 |
| BP-GPT [26] | FTC | Huth's | BLEU-1=21.28, METEOR=20.31 |
| BrainLLM (ours) | FTC | Huth's | BLEU-1=25.18, WER=92.02, METEOR=20.96 |
| | TC | Pereira's | BLEU-1=34.3, ROUGE-1=29.9, WER=75.8 |
| | TC | Huth's | BLEU-1=19.0, ROUGE-1=17.8, WER=89.2 |
| | TC | Narratives | BLEU-1=13.8, ROUGE-1=13.0, WER=92.4 |

**Table 11**: **Comparison of language generation performance (averaged across participants) of BrainLLM and the pre-construction followed by post-hoc selection model (Tang *et al.* [14]) in Huth's dataset.** Win rate indicates win rate versus PerBrainLLM. †/∗ denotes a significant difference with BrainLLM/PerBrainLLM using a Wilcoxon test with $q(FDR) < 0.5$ under the setting (with or without text prompt). The win rate for the Tang *et al.* [14]'s model is not available as the selection-based method can not get the possibilities of generating the perceived continuation. The work proposed by Tang *et al.* [14] utilizes a setting of generation without any text prompts while we utilize a setting with text prompts. Hence, we present their performance comparison in both settings.

| Setting | Model | BLEU-1(↑) | ROUGE-1(↑) | ROUGE-L(↑) | WER(↓) | Win rate |
|---|---|---|---|---|---|---|
| with text prompt | PerBrainLLM | 0.1668* | 0.1536* | 0.1474* | 0.9200* | 0.5000* |
| | Tang *et al.* [14] | 0.1675* | 0.1537* | 0.1483* | 0.9197* | - |
| | BrainLLM | **0.1899**† | **0.1780**† | **0.1709**† | **0.8916**† | **0.7667**† |
| without text prompt | PerBrainLLM | 0.0960* | 0.0817* | 0.0779* | 0.9703* | 0.5000* |
| | Tang *et al.* [14] | 0.0967†,* | 0.0818* | 0.0788†,* | 0.9700†,* | - |
| | BrainLLM | **0.1356**† | **0.1160**† | **0.1099**† | **0.9541**† | **0.8816**† |

**Table 12**: **Full-text reconstruction performance, excluding stop words, for a 10-minute-long story of "Where There's Smoke" in Huth's dataset.** $*$ indicates the performance difference between the pre-construction and post-hoc selection method proposed by Tang *et al.* [14] (denoted as "Classification") and BrainLLM is significant at $p < 0.05$ (one-sided t-test). Here, we evaluate "Classification" using its released decoding results (note that "Classification" with null inputs has not been released by Tang *et al.* [14]). Different from Table 2 in the main paper, we filter the reference content and decoded content through the NLTK stopwords library before calculating the evaluation metrics.

| Input | Method | BLEU-1 | WER | METEOR |
|---|---|---|---|---|
| Null | BrainLLM | 0.0147 | 1.0060 | 0.0509 |
| Subject 1 | Classification [14] | 0.0424* | 1.000* | 0.0707* |
| | BrainLLM | **0.0742** | **0.9622** | **0.1417** |
| Subject 2 | Classification [14] | 0.0615* | 0.9750* | 0.0807* |
| | BrainLLM | **0.0703** | **0.9718** | **0.1295** |
| Subject 3 | Classification [14] | 0.0704 | 0.9790* | 0.0897* |
| | BrainLLM | **0.0742** | **0.9685** | **0.1426** |

**Table 13**: **Performance of language generation without text prompt (averaged across participants) in different datasets.** The comparison between BrainLLM and PerBrainLLM are significant at $q(FDR) < 0.05$ (one-sided non-parametric test) on all datasets and metrics, respectively.

| **Dataset** | **Model** | **BLEU-1**(↑) | **ROUGE-1**(↑) | **ROUGE-L**(↑) | **WER**(↓) | **Win rate** (with PerBrainLLM) |
|---|---|---|---|---|---|---|
| Pereira's | PerBrainLLM | 0.0787 | 0.0553 | 0.0540 | 0.9726 | 0.5000 |
| | BrainLLM | **0.1025** | **0.0788** | **0.0749** | **0.9610** | **0.8885** |
| Huth's | PerBrainLLM | 0.0960 | 0.0817 | 0.0779 | 0.9703 | 0.5000 |
| | BrainLLM | **0.1356** | **0.1160** | **0.1099** | **0.9541** | **0.8816** |
| Narratives | PerBrainLLM | 0.1270 | 0.1133 | 0.1092 | 0.9328 | 0.5000 |
| | BrainLLM | **0.1320** | **0.1184** | **0.1145** | **0.9283** | **0.6728** |

**Table 14: Performance of language generation with LLM with different sizes of parameters in different datasets (averaged across participants).** As we focus on the performance comparison between BrainLLM and PerBrainLLM, we did not show experiments with StdLLM here. But you can find more results on StdLLM in our github repository (https://github.com/YeZiyi1998/Brain-language-generation). $*$ denotes a significant difference with BrainLLM using a Wilcoxon test with $q(FDR) < 0.5$ under the same model and the same dataset.

| Dataset | LLM backbone | Model | BLEU-1(↑) | ROUGE-1(↑) | ROUGE-L(↑) | WER(↓) |
|---|---|---|---|---|---|---|
| Pereira's | Llama-2 (7B) | StdLLM | 0.2415* | 0.2133* | 0.2096* | 0.8349* |
| | | PerBrainLLM | 0.3269* | 0.2815* | 0.2751* | 0.7783* |
| | | BrainLLM | **0.3432** | **0.2987** | **0.2878** | **0.7576** |
| | GPT-2-xl (1.5B) | PerBrainLLM | 0.2772 | 0.2340 | 0.2256 | 0.8246 |
| | | BrainLLM | 0.2814* | 0.2378* | 0.2292* | 0.8239* |
| | GPT-2-large (774M) | PerBrainLLM | 0.2605* | 0.2130* | 0.2057* | 0.8404* |
| | | BrainLLM | 0.2655 | 0.2182 | 0.2106 | 0.8395 |
| | GPT-2-medium (345M) | PerBrainLLM | 0.2100 | 0.1649* | 0.1605 | 0.8774 |
| | | BrainLLM | 0.2118 | 0.1672 | 0.1626 | 0.8779 |
| | GPT-2 (117M) | PerBrainLLM | 0.1866 | 0.1456 | 0.1426 | 0.8968 |
| | | BrainLLM | 0.1846 | 0.1445 | 0.1414 | 0.8973 |
| Huth's | Llama-2 (7B) | StdLLM | 0.1500* | 0.1360* | 0.1310* | 0.9200* |
| | | PerBrainLLM | 0.1668 | 0.1536 | 0.1474 | 0.9109 |
| | | BrainLLM | **0.1899** | **0.1780** | **0.1709** | **0.8916** |
| | GPT-2-xl (1.5B) | PerBrainLLM | 0.1708* | 0.1652* | 0.1581* | 0.9090* |
| | | BrainLLM | 0.1791 | 0.1729 | 0.1656 | 0.9022 |
| | GPT-2-large (774M) | PerBrainLLM | 0.1657* | 0.1584* | 0.1516* | 0.9132* |
| | | BrainLLM | 0.1762 | 0.1693 | 0.1616 | 0.9049 |
| | GPT-2-medium (345M) | PerBrainLLM | 0.1640* | 0.1549* | 0.1489* | 0.9140* |
| | | BrainLLM | 0.1667 | 0.1578 | 0.1514 | 0.9126 |
| | GPT-2 (117M) | PerBrainLLM | 0.1088* | 0.1059* | 0.0997* | 0.9516* |
| | | BrainLLM | 0.1096 | 0.1065 | 0.1011 | 0.9520 |
| Narratives | Llama-2 (7B) | StdLLM | 0.0953* | 0.0858* | 0.0829* | 0.9485* |
| | | PerBrainLLM | 0.1269* | 0.1211* | 0.1105* | 0.9311* |
| | | BrainLLM | **0.1375** | **0.1301** | **0.1209** | **0.9239** |
| | GPT-2-xl (1.5B) | PerBrainLLM | 0.1248* | 0.1171* | 0.1121* | 0.9340* |
| | | BrainLLM | 0.1298 | 0.1220 | 0.1168 | 0.9319 |
| | GPT-2-large (774M) | PerBrainLLM | 0.1202* | 0.1124* | 0.1074* | 0.9402* |
| | | BrainLLM | 0.1237 | 0.1159 | 0.1104 | 0.9401 |
| | GPT-2-medium (345M) | PerBrainLLM | 0.1056* | 0.0993* | 0.0950* | 0.9472* |
| | | BrainLLM | 0.1063 | 0.0999 | 0.0956 | 0.9463 |
| | GPT-2 (117M) | PerBrainLLM | 0.1099* | 0.1032* | 0.0980* | 0.9509* |
| | | BrainLLM | 0.1111 | 0.1047 | 0.0997 | 0.9506 |

**Table 15**: **Performance comparison among Tang et al., BP-GPT, and BrainLLM using base models with varying parameter sizes.** We used BLEU-1 and METEOR as metrics, as they are used across all these papers.

| **Method** | **Base model** | **BLEU-1** | | | **METEOR** | | |
|---|---|---|---|---|---|---|---|
| | | S01 | S02 | S03 | S01 | S02 | S03 |
| Tang et al. | GPT-2 (private) | 0.2331 | 0.2426 | 0.2470 | 0.1621 | 0.1677 | 0.1703 |
| BP-GPT | GPT-2 (public, small) | 0.2159 | 0.2111 | 0.2113 | **0.2082** | 0.1976 | 0.2034 |
| BrainLLM | GPT-2 (public, small) | 0.2364 | 0.2164 | 0.2297 | 0.2041 | 0.1982 | 0.2062 |
| BrainLLM | GPT-2 (public, xl) | **0.2539** | **0.2518** | **0.2497** | 0.2078 | **0.2031** | **0.2180** |

**Table 16**: **Full-text reconstruction results with BrainLLM and Tang *et al.* [14]'s method for subject 1 in Huth's dataset.** Blue text indicates the generation output and the perceived continuation are exact match. These samples were selected from participants 1, 2, and 3. The results of Tang *et al.* [14]'s method are inherited from their paper, refer to our repository (https://github.com/YeZiyi1998/Brain-language-generation) for more reconstruction results among different participants.

| Reference | BrainLLM | Tang et al.'s method |
|---|---|---|
| i had no shoes on i was crying i had no wallet but i was ok because i had my cigarettes | she **was** the first person **i** met in **my** first year of college **i was** in a relationship with **my** boyfriend and **i** | she said she **was** a little stressed out **because** she wasn't doing anything wrong and **had** a lot of anxiety issues **but i had** been |
| and i didn't want any part of freedom if i didn't have my cigarettes when you live with someone who has a temper a very bad temper a | had **a** lot **of** friends **and** family **who** had been **very** kind to me **and i** decided to go for it **and i** went | watching the news **and** realized that her mom was the most important thing to me **and i** was not **a** fan **of** this guy she was **a** nice girl **i** loved |
| very very bad temper you learn to play around that you learn this time i'll play possum and next time i'll | **to** the hospital **and** they said i can't do **that** i don't know if i'm going **to** be a better person i would be if i were | her **very** much but i couldn't let her go without making it clear i wanted a relationship she would say no **to** everything **and** be willing **to** |
| just be real nice or i'll say yes to everything or you make yourself scarce or you run and this was one of the times when you just run and as | **to** die i would still **be** able **to** do it **and** i felt like it **was the** right thing **to** do **and** i **was** like well i don't know what i'm gonna | deal with anything **just as** long **as** it didn't mean something she **was** afraid **of** i did it a lot **of times** but never like **this and** |
| i was running i thought this was a great place to jump out because there were big lawns and there were cul de sacs and sometimes he would come after me and drive and yell stuff at me to get back in get back in | do is **i** go **out to** the car **and i** got **out** of the car **and** into the house **and i** went **to** the bathroom **and i was** like oh my god **i** can't | now **i** see how she can make it work with **a** single phone call **to** the hospital my first instinct is **to run** over **and** kick her **out** of the room **and** say no you can |
| and i was like no i'm out of here this is great and i went and hid behind a cabana and he left and i had my cigarettes and uh i started to walk in this | do **this i** can't believe **i'm** gonna die so **i** go back **to** the car **and i** got **to** the end | do **this i** refuse **to** go back there so **i** sit down at the dining table **and i** ask him what **is** the point **of** having the |
| beautiful neighborhood it was ten thirty at night and it was silent and lovely and there was no sound except | of my life **and** i went back to my room **and** i **was** like oh my god this is | house built on the beach **at night it was** a **beautiful** day i **was** going to stay **at** the house of my grandparents that **was** |
| for sprinklers ch ch ch ch ig ch ch ch ch ig and i was enjoying myself | the first time **i**'ve ever been in a place like you know | near a beach it **was** a perfect day so **i** |
| and enjoying the absence of anger and enjoying these few hours i knew i'd have of freedom and just to perfect it i thought i'll have a smoke and | **i** was in **the** middle **of a** very bad year for me **and i** had **to** go back **and** get my degree **and i** got **a** job **and i** went | was **just** being nice **to** my friends **i** didn't get much **of a** chance **to** do anything until later that evening at am **and i** decided **to** take my phone |

| | | |
|---|---|---|
| then it occurred to me with horrifying speed i don't have a light just then as if in answer i see a figure up ahead | **to** college and **i** got **a** job and i'm not sure **if** you're gonna be **in** the same room **with** her and **i** was like oh my god this is the best | out **i** was worried that my battery had died or something **as i** got **it i** looked around and saw **a** red **light** coming |
| who is that it's not him ok they don't have a dog who is that what uh what are they doing out on this suburban street and the person comes closer and i could see it's a woman | job i've ever had **and** i'm **not** sure if you know **this is the** first time i've ever been in **a** situation like **this and i** was **on the** ground **and** | from **the** house my mom called **out i** know **who that is i** said we got there **a** few minutes before **him and** his girlfriend came to **a** stop in |
| and then i can see she has her hands in her face oh she's crying and then she sees me and she composes herself and she gets closer and i see she has no | **then i** hear a loud pop **and i** looked up **and** there was this guy who was a friend of the family came to **see me and i** was like | front of us the girl had **her** arms out **and her** head **in** my direction **she** looked scared **and** the guy just kept staring at **me she** turned around **and i** saw |
| shoes on she has no shoes on and she's crying and she's out on the street street i recognize her though i've never met her and just as she passes me she | oh my god **i** am so scared **i** don't even know what to do with my life **i** don't know what to say so **i** said yes **and i** was like | **her** face **she** was in a black suit **i just** had a bad feeling that **she** knew **me** from somewhere but **she** didn't know **me** at all **she** looked |
| says you got a cigarette and i say you got a light and she says damn i hope so and then sh first she digs into her cutoffs in the | well i'm not sure **i** don't know what to **say so i** said okay well i'm gonna go to **a** party **and i** | at me **and** asked if **i** wanted **a** beer but **i** told **her i** couldn't **so i got** one out of my backpack **and** poured it down |
| front nothing and then digs in the back and then she has this vest on that has fifty million little pockets on it and she's checking and checking and it's looking bad it's looking very bad | was like oh my god i'm **in the** shower **and** i had to put **on** a pair of pants **and** a shirt **that** was | her shirt **the** top button was ripped **and** there was a piece of paper stuck **in** there with a bunch of random numbers **and** words i couldn't understand at all so i |
| she digs back in the front again deep deep and she pulls out a pack of matches that had been laundered at least once ukgh we open | **a** little too much for me so i put on **a** white shirt **and a** pair **of** pants **and a** shirt um **and** i was | got down to **the** first two boxes **and pulled the** top off one was filled with **a** pile **of** money **that** was still **in** there so |
| it up and there is one match inside ok oh my god this takes on it's like nasa now we got to like oh how are we gonna do it ok and we we hunker down | **like oh my god** i don't know what i'm **gonna do and** i think that was the first time i had **to do it and** i was **like oh** | he took **it** back **and** said sorry about **this** i don't think anyone can help you **now it's** all done **now** so **it** would be better **to** be |
| we crouch on the ground and where's the wind coming from we're stopping i take out my cigarettes let's get the cigarettes ready oh my brand she says not surprising and | **my** god i'm in **the** middle of a field **and** then **i** went back to **the** car **and i** was like **oh my** god **i** have to tell you i'm **not** | able to see **the** light **from the** sky then it's **my** turn to help him pick up his shoes **i** suggest **taking** them off as he is |

| | | |
|---|---|---|
| we both have our cigarettes at the ready she strikes once nothing she strikes again yes fire puff inhale mm sweet kiss of that cigarette | gonna be able to do it and then i get out **of the** car and i'm sitting in **the** back seat **of the** car and i | about to fall so he goes for it he drops them and they are immediately shot and blown to pieces as he walks |
| and we sit there and we're loving the nicotine and we both need this right now i can tell the night's been tough immediately we start to reminisce | got **to the** end of that day **i** was in **the** middle of it **and i** was like well i'm going **to tell** you | away **and i sit** down with my wife **to** be able **to** see what happened **the** whole time my husband was at **the** hospital for about two weeks |
| about our thirty second relationship i didn't think that was gonna happen me neither oh man that was close oh i'm so lucky i saw you yeah then she | a story **about** the time **i was** in high school and **i was** a good kid **i** mean you're not **gonna** be able to do it | while his wife **was** in surgery when he called **me i** said **you** know what **you** did right and **that was** when **i** got |
| surprises me by saying what was the fight about and i say wha what are they all about and she said i know what you mean she said was it a bad one and and i said | **and i was** like well **i** don't **know what** to tell **you and i said** well **you know i** don't think you're going to get married **and i was** | an email from **the** girl asking **me** if **i** had heard of this **i said** no **i** did not **the** reply **was you** don't **know** of course |
| you know like medium she said oh and we start to trade stories about our lives we're both from up north we're both kind of newish to | **like oh** my god i was so nervous **and** excited **about** this new job i had was as a young man i was dating a guy who | not **and we** laughed **and** i got a call **from** a friend in the same town **we lived** in that had a small local |
| the neighborhood this is in florida we both went to college not great colleges but man we graduated and i'm actually finding myself a little jealous of her because she has this really cool | was **a** friend **of** my mom's **and** my dad's house was on **the** other side **of the** room **and** i was so excited **to** get my first | **college** on **the** east coast **and** was an engineering school with **a great** program they were pretty good people **but** there was one who seemed **really** into it **and** started talking about his |
| job washing dogs she had horses back home and she really loves animals and she wants to be a vet and i'm like man you're halfway there | **job** as **a** waitress i was working at the time **and** i was **like** oh my god i don't know what **to** do with | degree in art history he **had a** phd **and** he **wanted to** teach **a** new language i told him no way he should **be** |
| i'm a waitress at an ice cream parlor so um that's not i don't know where i want to be but i know it's not that and then it gets a little deeper cg | **it um and i** was like oh my god **i'm so** nervous **i don't know** what **to** do with **it and i** was like oh my god **i** | working in **an** engineering lab with **a** phd **but i** didn't say **that i** wasn't happy about **it and i** was in the middle of |
| and we share some other stuff about what our lives are like things that i can't ever tell people at home this girl i can tell her the really ugly stuff and she | have to go **home and i** went to see **her and she** said you know **what i** think **about** you **and i** know | a presentation with **some people** who were coming up for their first visit to a new place **i** had already told **her i** wanted to be friends but **she** seemed to |

| | | |
|---|---|---|
| still understands how it can still be pretty she understands like how nice he's gonna be when i get home and how sweet that'll be | you're not **gonna be** able to help you with that but **i** don't know what to do **and i** just couldn't do **it and** | not feel the same way about **it** the thing is **when** you find out you're not good enough for someone to love you **and** |
| we are chain smoking off each other oh that's almost out come on and we we go through this entire pack until it's gone and then i say you know what uh this is a little funny but you're gonna | i'm like **oh i** don't **know what** i'm **gonna** do **is** i'll be able to get **out** of the car **and then i** got to the end of | **you** just have to fight the urge to throw the ring back in the box **and** take your pick of the two **and** set them free **but i** can't **i** need |
| have to show me the way to get home because although i'm twenty three years old i don't have my driver's license yet and i just jumped out right when i needed to and she says well why don't you come back to my house and i'll give you | **my** life so **i** go **to the** store **and i** went **to** college **and i** got a job at **the** university **and i** was like oh **my** god **i have to** go **and** | **to** ask **you** something about **my** childhood **i** had **to get my license to** drive so **my** mom could **have me out** of **the house and she** wanted **me to** go with her **to** visit **my** dad |
| a ride i say ok great and we start walking and uh we get to this um lots of uh lights and uh the roads are getting | **i** said okay **and** he **says** well you know **i** don't really want **to** do it but **i** had **to** | so **we** left **and** got back home **and** it was then that **i** noticed something was different about **the** way **the light** was |
| wider and wider and there's more cars and i see um lots of stores you know laundromats and dollar stores and emergecenters and | get out **of** the **car and i** got out **of** the **car and i** got out **of** the **car and i** got | changing around me **and i** looked up **and** saw a tall building with a few towers **and** a white flag flying above it **and** then |
| then we cross over us one and uh she leads me to some place and i think no but yes carl's efficiency | in the car **and i** was like oh my god this is the first time i've ever seen you **and i** was like well **i** don't know what **to** do | **we** came across a town about miles from our house **and i** thought oh god it was my grandmother the |
| apartments this girl lives there and it's horrible and it's lit up so bright just to illuminate the horribleness of it it's the kind of place where you drive your car right up and the door's | with **it and** i think **it's** a good thing i think **it's** a good thing i guess is that i'm a big fan **of the** old | old lady from **the** church that was **so** very special **to** us but **it** was very sad because **it** meant that she had a death certificate she was |
| right there and there's fifty million cigarette butts outside and there's like doors one through seven and you know behind every single door there's some horrible misery going on there's someone crying or drunk | black **and** white tv set in the living room of my parents house **and** i was the only **one** in my | **on** the front page of **every** newspaper **and** it was just the top of the times which meant that **there** were stories of her being beaten at her job **and** having a |
| or lonely or cruel and i think oh god she lives here how awful we go to the door door number four and she very very quietly | family **i** was **the** only girl in **the** whole world **and i** was like well **i** don't know what i'm gonna do is **i go to the** hospital **and** | boyfriend who beat her up but he wasn't that bad **to** begin with so **i** went **to the** cops **i** had **to** walk out of there **and** |

| | | |
|---|---|---|
| keys in as soon as the door opens i hear the blare of television come out and on the blue light of the television the smoke of a hundred cigarettes in that little crack of light | **i** went back to **the** car **and i** got **out of the** car **and** into **the** back seat **of the** car **i** was sitting **in the** back **of** my head **and** | take my chances **and i** got into **a** car **that** was sitting there **the** passenger seat was full **of** beer bottles **and the** front windshield had glass **in** it **and** |
| and i hear the man and he says where were you and she says never mind i'm back and he says you alright and she says yeah i'm alright | **i'm** like what **the** fuck is wrong with **you and i'm** like well **i** don't know what to **say** so **i** tell **you** what **i'm** gonna | my mother was screaming at my father **and saying** oh no **you** aren't leaving us **he** said well why not **i** looked |
| and then she turns to me and says you want a beer and he says who the fuck is that and she pulls me over and he sees me and he says oh hey i'm not a threat | **say is** it okay if i go out with him **and** i said well **you** know **i'm not** sure i don't know what **to** | at my dad **who** was smiling i told my mom **to** call him back **and** when **he** finally answered **she** said no thanks my dad |
| just then he takes a drag of his cigarette a very hard hard drag you know the kind that makes the end of it really heat up hot hot hot and long and it's a little scary and | do so i went into **the** bathroom **and** i was in there for **a** while **and then** i would go to **the** hospital **and** get **the** best care i could get **and** i had to **take** | had some sort **of** breakdown **and just** threw **up** for days **it** was **a very** serious form **of** depression **that** was going around **and** i had to put |
| i follow the cigarette down because i'm afraid of that head falling off and i'm surprised when i see in the crook of his arm a little boy sleeping | **off** my shoes **and i** put them on **the** floor **and i** was like oh my god **i'm** so glad **i** didn't have to | my hands up to hide **the** fact **that** it hurt to have it pulled up **the** skin on **the** side **of** my face **and** over my eye |
| a toddler and i think and just then the girl reaches underneath the bed and takes out a carton and she taps out the last s pack of cigarettes in there | worry about my dad **and i** was like oh my god i'm **in the** shower **and i** get **in the** car **and** we drove **out** to **the** | my dad said what is that he walked up to my father grabbed **the** shotgun from his side **and** started loading it with |
| and on the way up she kisses the little boy and then she kisses the man and the man says again you alright and she says yeah i'm just gonna go out and smoke with her and so | beach **and** there's this guy **and** he's like oh my god i can't believe you're **going** to be | rounds i immediately pulled my brother to me **and** hugged him i **then** asked my sister if **she** could stay **with** us we all left to **go** get our cars **and** |
| we go outside and sit amongst the cigarette butts and smoke and i say wow that's your little boy and she says yeah isn't he beautiful and i say yeah he is he is beautiful | a couple of days later **i** get a call from my dad **and i** was like well i'm not sure **i** don't know what to **say** but **i** | drove to **the** beach at am on **the** way back **he** said **i** can't believe this **i** don't understand it i'm like oh man you must be |
| he's my light he keeps me going she says we finish our cigarettes she finishes her beer i don't have a beer cause i can't go home | know you're not **going** to like this but **i** think it was the first time **i** had sex with you and **i** think you're | really special if you're the best thing in **my** life and **i** can barely speak **i** will probably never **have** sex again for fear of |

| | | |
|---|---|---|
| with beer on my breath and she goes inside to get the keys she takes too long in there getting the keys and i | gonna have **to** do a lot of work **on the** car **and i** got out of **the** car **and** | becoming addicted **to the** stuff **and** then it **gets** worse when **she** comes out of it **i** start **to** worry that something is |
| think something must be wrong and she comes out and she says look i'm really sorry but um like we don't have any gas in the car it's already on e and he needs to get to work in the morning and um | i got **out** of **the car and** i went **to the** bathroom **and** i went **in** there **and** i was **like** oh my god i can't believe **i'm having** a baby **and** i was **like** | **wrong but** then **she says to** me hey do you **think she** can afford **to** pay rent **on** time **to** a school for her kids **to** go **to and** |
| i you know i i'm gonna be walk to work as it is so what i did was though here look i drew out this map for you and you're really you're like a mile and a half from home and um if you walk three streets over you'll be back on that pretty street | well **i** don't **know what to** do **so i** told him **that i was** going **to** do **it and** then **i** got **a** call **from** one of the guys who had been in the hospital **for a** | she would just say oh sorry **i did** the math **on this** one **i** will send her **a** link **to a** different site in the same time period **to** see how far **back** |
| and you just take that and you'll be fine and she also has wrapped up in toilet paper seven cigarettes for me a third of her pack i note and a new pack of | couple **of** days **and** then **i** had to put on **a** pair **of** tiny white leering eyes **and** my hair was done **and i** had to get my | **she** gets so **i** do this too **i** put **a** bunch **of** photos **in** an envelope with **a** few other stuff **i** brought **a** box **of** |
| matches and she tells me good bye and that was great to meet you and how lucky and that was fun and you know let's be friends | hair done **and** then i go home **and** i **tell** my mom i love her so much but i just couldn't do it | them **and** he thanked **me** again then we started **to** talk about our life **and** the family he **was** from **and** i |
| and i say yeah ok and i walk away but i kind of know we're not gonna be friends i might not ever see her again and i kind of | **and** i'm like well **i** don't **know** what to do so **i** go to university **and i** got a job at the | said yes **and** then **i** got angry when **i** thought about it because **i** wasn't sure what was happening **i** didn't really care at all |
| know i don't think she's ever going to be a vet and i cross and i walk away and maybe this would've seemed like a visit from my possible future and scary but it | university **and i** get **a** job at the club **and** then **i** went back **to my** room **and i** sat in **my** room for hours on end **and i** was | until **i** saw **it** was the girl **from my** dreams that was driving down the road **and i** started **to** notice that the car was **a** bit older than **my** own **i** couldn't |
| kind of does the opposite on the walk home i'm like man that was really grim over there and i'm going home now to my nice boyfriend | **like** oh **my** god **i'm** so sorry i don't know what i **was going to** do a lot **of** things **that** i didn't want **to** be | make it out clearly so i yelled hey you have **to** stop i just saw a **man that** i knew in **the** past who **was** very physically |

| | | |
|---|---|---|
| and he is gonna be so extra happy to see me and we have a one bedroom apartment and we have two trees and there's a yard and we have this jar in | **a** girl **and** i was **so happy and** i was **so** excited **and** i was like oh my god **this is** the first time i've | abused by his wife she had him committed **and** was now living **in** his **bedroom** where **he** had **a** couch **and** tv the **apartment** was about feet long **and** had |
| the kitchen where there's like loose money that we can use for anything like we would never ever run out of gas and um i don't have a baby you know so i can leave whenever i want | **ever** been to **and i** was **like** oh my god **i** can't believe you're | two bathrooms **and a** huge closet to store **the** clothes **i** didn't **have** any **money** or food because **i** wasn't hungry **i** was lucky my parents didn't lock me up **so** |
| i smoked all seven cigarettes on the way home and people who have never smoked cigarettes just think ick disgusting and poison | not going to see him again **the** next day **and** you know **i think** it's a really good question **and i** don't know what to do | **i just** started drinking **all the** time **the** day before thanksgiving **and** my mom told me that **the** reason she doesn't like alcohol is because it's addictive **i** don't |

**Table 17**: **Statistics of the LLMs adopted in our experiments.** These statistics are reported according to the original paper [5, 31] and the public sourced repositories (https://huggingface.co/meta-llama/Llama-2-7b and https://huggingface.co/gpt2).

| **Model** | **#Parameters** | **#Transformer layers** | **Embedding size** | **Vocabulary size** | **Quantization** | **#Max input tokens** |
|---|---|---|---|---|---|---|
| Llama-2 | 7B | 32 | 4,096 | 32,000 | float16 | 4,096 |
| GPT-2-xl | 1.5B | 48 | 1,600 | 50,257 | float32 | 1,024 |
| GPT-2-large | 774M | 36 | 1,280 | 50,257 | float32 | 1,024 |
| GPT-2-medium | 345M | 24 | 1,024 | 50,257 | float32 | 1,024 |
| GPT-2 | 117M | 12 | 768 | 50,257 | float32 | 1,024 |

**Table 18**: Win rate of BrainLLM versus PerBrainLLM across different selections of the Brain adapter structures in Huth's dataset.

| **Structure** | **MLP+pos** | **MLP** | **concat+MLP** | **RNN** | **Linear** |
|---|---|---|---|---|---|
| Win rate | **0.7893** | 0.7782 | 0.6826 | 0.6755 | 0.7155 |

**Table 19**: Language similarity metrics of BrainLLM with different training protocols with the backbone LLM GPT2-xl in Huth's dataset.

| **Training protocol** | **BLEU-1** | **ROUGE-1** | **ROUGE-L** | **WER** |
|---|---|---|---|---|
| Full parameter fine-tuning | 0.1331 | 0.1228 | 0.1180 | 0.9342 |
| Combined | 0.1672 | 0.1611 | 0.1523 | 0.9197 |
| Prompt-tunning | **0.1791** | **0.1729** | **0.1656** | **0.9022** |

**Table 20**: Overall statistics of fMRI datasets.

| **Dataset** | **Stimuli** | **#Partic ipants** | **#Total Duration** | **#Duration per participant** | **#Total TRs** | **#TRs per participant** | **#Total words** | **#Words per participant** |
|---|---|---|---|---|---|---|---|---|
| Pereira's | visual | 5 | 7.0 h | 1.4 h | 3135 | 627 | 38650 | 7730 |
| Huth's | auditory | 8 | 3.5 days | 10 h | 122992 | 15374 | 427296 | 53412 |
| Narratives | auditory | 28 | 21.0h | 45 min | 48496 | 1732 | 230460 | 8231 |

**Table 21**: Win rate of BrainLLM versus PerBrainLLM across different selections of the learning rate and reduction dimension in Huth's dataset. We set the learning rate to $1 \times 10^{-4}$ and choose the reduction dimension $c$ as 1,000 which offers the best performance while balancing computational efficiency. We then consistently apply these parameters across all datasets and in all further analyses.

| **Learning rate** | $1e^{-3}$ | $1e^{-4}$ | $1e^{-5}$ | $1e^{-6}$ |
|---|---|---|---|---|
| Win rate | 0.7334 | **0.7893** | 0.7746 | 0.7240 |

| **Reduction dimension** | 500 | 1,000 | 2,000 | 4,000 |
|---|---|---|---|---|
| Win rate | 0.7532 | **0.7893** | 0.7813 | 0.7767 |

**Table 22**: **Language generation performance averaged across participants in different datasets, excluding stop words.** Different from Table 2 in the main paper, we filter the reference content and decoded content through the NLTK stopwords library before calculating the evaluation metrics. $*$ indicates that the difference between BrainLLM and PerBrainLLM is significant at $q(FDR) < 0.05$ (one-sided non-parametric test).

| Dataset | Model | BLEU-1(↑) | ROUGE-1(↑) | ROUGE-L(↑) | WER(↓) |
|---|---|---|---|---|---|
| Huth's | PerBrainLLM | 0.1012* | 0.1130* | 0.1125* | 0.9458* |
| | BrainLLM | **0.1195** | **0.1353** | **0.1344** | **0.9242** |
| Pereira's | PerBrainLLM | 0.2708* | 0.2536* | 0.2466* | 0.8729* |
| | BrainLLM | **0.2975** | **0.2705** | **0.2604** | **0.8437** |
| Narratives | PerBrainLLM | 0.1002* | 0.1034* | 0.1034* | 0.9596* |
| | BrainLLM | **0.1107** | **0.1145** | **0.1145** | **0.9523** |

**Table 23**: **Selected examples of language generation with BrainLLM and PerBrainLLM for showing the relationship between different measurements.**

| **Text prompt** | **Perceived continuation** | **Generation with BrainLLM** (surprise) | **Generation with PerBrainLLM** (surprise) |
|---|---|---|---|
| Scrubbing a wound with soap or alcohol delays healing, which | increases the risk of infection. | can lead to infection. (0.5653) | can lead to infection. (0.6313) |
| i started looking around this room and thinking about what they would think about me | when i quit they | and what they would think about each other and(3.8415) | and i thought about what they would think about(4.8872) |
| Salmon is a fish that migrates from fresh water to | the ocean and back to spawn. | the sea and back.(1.0145) | the sea to spawn.(1.3141) |
| the water and by golly mike was not gonna let his hands go under that water | and i realize | he was gonna make sure we all got(4.6175) | so i'm standing there and he's like what(2.9743) |
| a and i'm just watching and we're | slowly starting to fall towards | driving and then all of a sudden we're stopped at(3.7490) | just watching and i'm not sure what we're supposed to(4.7661) |

**Table 24**: **Language generation performance averaged across participants in different datasets.** The difference between BrainLLM and PerBrainLLM/StdLLM are significant at $q(FDR) < 0.05$ (one-sided non-parametric test) on all datasets and metrics, respectively.

| Dataset | Model | BLEU-1(↑) | ROUGE-1(↑) | ROUGE-L(↑) | WER(↓) |
|---|---|---|---|---|---|
| Pereira's | StdLLM | 0.2415 | 0.2133 | 0.2096 | 0.8349 |
| | PerBrainLLM | 0.3269 | 0.2815 | 0.2751 | 0.7783 |
| | BrainLLM | **0.3432** | **0.2987** | **0.2878** | **0.7576** |
| Huth's | StdLLM | 0.1500 | 0.1360 | 0.1310 | 0.9200 |
| | PerBrainLLM | 0.1668 | 0.1536 | 0.1474 | 0.9109 |
| | BrainLLM | **0.1899** | **0.1780** | **0.1709** | **0.8916** |
| Narratives | StdLLM | 0.0953 | 0.0858 | 0.0829 | 0.9485 |
| | PerBrainLLM | 0.1269 | 0.1211 | 0.1105 | 0.9311 |
| | BrainLLM | **0.1375** | **0.1301** | **0.1209** | **0.9239** |

**Table 25**: Experimental results of the full-text construction task for a perceived story "where there's smoke" with a range of language similarity metrics in three subjects of Huth's dataset. (1) A floor for each metric was computed by scoring the mean similarity between the actual stimulus words and a sequence generated from a language model without using any brain data ("null"). Here Tang *et al.* [14] uses a private language model which is trained in a corpus constructed with Reddit stories and is similar to the perceived story content. On the other hand, we use a publicly available language model GPT2-xl which is trained in a general corpus and therefore shows worse performance when compared to Tang *et al.* [14] when no brain input is given. (2) When given brain input, the proposed BrainLLM outperforms Tang *et al.* [14] in all language similarity metrics. A pair-wise t-test shows significant improvements are observed particularly in METEOR ($p = 3e^{-5}$), and in WER ($p = 0.03$). (3) We also test a more fair control with the brain input permutated. The experimental results demonstrate that our method significantly outperforms the control model in metrics of BLEU-1 ($p = 3e^{-4}$), and WER ($p=5e^{-4}$). (4) A ceiling for each metric was computed by manually translating the actual stimulus words into Mandarin Chinese, and automatically translating the words back into English using a state-of-the-art machine translation system. The numbers are inherited from Tang *et al.* [14]'s paper.

| **Input** | **Method** | **Metrics** | | |
|---|---|---|---|---|
| | | **BLEU-1**(↑) | **WER** (↓) | **METEOR**(↑) |
| Null (without brain input) | Tang *et al.* [14] | 0.1908 | 0.9637 | 0.1323 |
| | GPT2-xl | 0.1417 | 0.9569 | 0.1181 |
| Permutated brain input of Subject 1 | Tang *et al.* [14] | 0.1967 | 0.9703 | 0.1542 |
| | BrainLLM | 0.2363 | 0.9499 | 0.1995 |
| Brain input of Subject 1 | Tang *et al.* [14] | 0.2331 | 0.9407 | 0.1621 |
| | BrainLLM | **0.2539** | **0.9158** | **0.2078** |
| Permutated brain input of Subject 2 | Tang *et al.* [14] | 0.2016 | 0.9761 | 0.1586 |
| | BrainLLM | 0.2161 | 0.9545 | 0.1988 |
| Brain input of Subject 2 | Tang *et al.* [14] | 0.2426 | 0.9354 | 0.1677 |
| | BrainLLM | **0.2518** | **0.9259** | **0.2031** |
| Permutated brain input of Subject 3 | Tang *et al.* [14] | 0.2173 | 0.9576 | 0.1695 |
| | BrainLLM | 0.2068 | 0.9755 | 0.2011 |
| Brain input of Subject 3 | Tang *et al.* [14] | 0.2470 | 0.9243 | 0.1703 |
| | BrainLLM | **0.2497** | **0.9190** | **0.2180** |
| Mandarin | machine translation | 0.4363 | 0.7459 | 0.3991 |

# References


1. Pereira, F. *et al.* Toward a universal decoder of linguistic meaning from brain activation. *Nature communications* **9,** 963 (2018).
2. LeBel, A. *et al.* A natural language fMRI dataset for voxelwise encoding models. *Scientific Data* **10,** 555 (2023).
3. Nastase, S. A. *et al.* The "Narratives" fMRI dataset for evaluating models of naturalistic language comprehension. *Scientific data* **8,** 250 (2021).
4. Luo, Y., Xu, M. & Xiong, D. Cogtaskonomy: Cognitively inspired task taxonomy is beneficial to transfer learning in NLP. In *Proceedings of the 60th Annual Meeting of the Association for Computational Linguistics* **1** (2022), 904–920.
5. Touvron, H. *et al.* Llama: Open and efficient foundation language models. *arXiv preprint arXiv:2302.13971* (2023).
6. Liu, X. *et al.* GPT understands, too. *AI Open* **5,** 208–215 (2023).
7. Cho, J., Nam, G., Kim, S., Yang, H. & Kwak, S. Promptstyler: Prompt-driven style generation for source-free domain generalization. *Proceedings of the IEEE/CVF International Conference on Computer Vision* **1,** 15702–15712 (2023).
8. Feghhi, E., Hadidi, N., Song, B., Blank, I. A. & Kao, J. C. What Are Large Language Models Mapping to in the Brain? A Case Against Over-Reliance on Brain Scores. *arXiv preprint arXiv:2406.01538* (2024).
9. Huang, S. *et al.* Language is not all you need: Aligning perception with language models. In *Advances in Neural Information Processing Systems* **36** (2024).
10. Duan, Y., Chau, C., Wang, Z., Wang, Y.-K. & Lin, C.-t. Dewave: Discrete encoding of eeg waves for eeg to text translation. In *Advances in Neural Information Processing Systems* **36** (2024).
11. Fathullah, Y. *et al.* AudioChatLlama: Towards General-Purpose Speech Abilities for LLMs. In *Proceedings of the 2024 Conference of the North American Chapter of the Association for Computational Linguistics: Human Language Technologies* **1** (Association for Computational Linguistics, Mexico City, Mexico, 2024), 5522–5532.
12. Chu, Y. *et al.* Qwen2-audio technical report. *arXiv preprint arXiv:2407.10759* (2024).
13. Tikochinski, R., Goldstein, A., Meiri, Y., Hasson, U. & Reichart, R. Incremental accumulation of linguistic context in artificial and biological neural networks. *Nature Communications* **16,** 803 (2025).
14. Tang, J., LeBel, A., Jain, S. & Huth, A. G. Semantic reconstruction of continuous language from non-invasive brain recordings. *Nature Neuroscience* **26,** 1–9 (2023).
15. Radford, A., Narasimhan, K., Salimans, T. & Sutskever, I. *Improving language understanding by generative pre-training* OpenAI. https://cdn.openai.com/research-covers/language-unsupervised/language_understanding_paper.pdf. 2018.
16. Toneva, M. & Wehbe, L. Interpreting and improving natural-language processing (in machines) with natural language-processing (in the brain). In *Advances in Neural Information Processing Systems* **32** (2019), 14928–14938.
17. Toneva, M. *Bridging Language in Machines with Language in the Brain* PhD thesis (Carnegie Mellon University, 2021).
18. Schrimpf, M. *et al.* The neural architecture of language: Integrative modeling converges on predictive processing. *Proceedings of the National Academy of Sciences* **118,** e2105646118 (2021).
19. Anderson, A. J. *et al.* Deep artificial neural networks reveal a distributed cortical network encoding propositional sentence-level meaning. *Journal of Neuroscience* **41,** 4100–4119 (2021).
20. Jo, H. *et al.* Are EEG-to-Text Models Working? *arXiv preprint arXiv:2405.06459* (2024).
21. Wang, Z. & Ji, H. Open vocabulary electroencephalography-to-text decoding and zero-shot sentiment classification. *Proceedings of the AAAI Conference on Artificial Intelligence* **36,** 5350–5358 (2022).
22. Xi, N. *et al.* UniCoRN: Unified Cognitive Signal ReconstructioN bridging cognitive signals and human language. In *Proceedings of the 61st Annual Meeting of the Association for Computational Linguistics* **1** (2023), 13277–13291.

23. Yang, Y., Duan, Y., Zhang, Q., Xu, R. & Xiong, H. Decode neural signal as speech. *arXiv preprint arXiv:2403.01748* (2024).
24. Zhao, X. *et al.* MapGuide: A Simple yet Effective Method to Reconstruct Continuous Language from Brain Activities. *Proceedings of the 2024 Conference of the North American Chapter of the Association for Computational Linguistics: Human Language Technologies (Volume 1: Long Papers),* 3822–3832 (2024).
25. Yin, C., Ye, Z. & Li, P. Language Reconstruction with Brain Predictive Coding from fMRI Data. *arXiv preprint arXiv:2405.11597* (2024).
26. Chen, X., Du, C., Liu, C., Wang, Y. & He, H. Open-vocabulary Auditory Neural Decoding Using fMRI-prompted LLM. *arXiv preprint arXiv:2405.07840* (2024).
27. Rainey, S., Martin, S., Christen, A., Mégevand, P. & Fourneret, E. Brain recording, mind-reading, and neurotechnology: ethical issues from consumer devices to brain-based speech decoding. *Science and engineering ethics* **26,** 2295–2311 (2020).
28. Mecacci, G. & Haselager, P. Identifying criteria for the evaluation of the implications of brain reading for mental privacy. *Science and Engineering Ethics* **25,** 443–461 (2019).
29. Défossez, A., Caucheteux, C., Rapin, J., Kabeli, O. & King, J.-R. Decoding speech perception from non-invasive brain recordings. *Nature Machine Intelligence,* 1–11 (2023).
30. He, S., Zhu, J., He, P. & Lyu, M. R. Loghub: A large collection of system log datasets towards automated log analytics. *arXiv preprint arXiv:2008.06448* (2020).
31. Radford, A. *et al.* Language models are unsupervised multitask learners. *OpenAI blog* **1,** 9 (2019).
